# Supplementary material for: Field-theoretic functional renormalization group formalism for non-Fermi liquids and its application to the antiferromagnetic quantum critical metal in two dimensions
Source: arXiv:2208.00730 source file (2023-01-06)
Supplement: Supplementary file 1 [file appendixBeta_Final.tex]

\section{Beta functionals for shifted four-fermion couplings 
\attention : To be removed
}
\label{sec:shiftedffc}

With
\begin{equation}
{\lambda}^{' \mathrm{I};\spmqty{\alpha & \beta \\ \delta & \gamma}}_{\spmqty{k_1 & -k_1 \\ k_2 & -k_2}} = \frac{1}{\sqrt{{V}_{F,K_1}{V}_{F,K_2}}}\left({\lambda}^{\mathrm{I};\spmqty{\alpha & \beta \\ \delta & \gamma}}_{\spmqty{k_1 & -k_1 \\ k_2 & -k_2}} - \frac{2 \mathsf{T}^{\alpha \beta}_{\delta \gamma}}{N_f}{\mathsf{D}}(k_1; k_2)  \pmqty{0 & 1 \\ 1 & 0} \right),
\end{equation}
\eq{eq:betabigmatrixsimple_main0} can be written as
\begin{equation}
\begin{aligned}
\frac{\partial}{\partial\ell}{\lambda}^{' \mathrm{I}; \spmqty{\sigma_1 & \sigma_2 \\ \sigma_4 & \sigma_3}}_{\spmqty{p & -p \\ k & -k }} = & 
- {\lambda}^{' \mathrm{I}; \spmqty{\sigma_1 & \sigma_2 \\ \sigma_4 & \sigma_3}}_{\spmqty{p & -p \\ k & -k }}
%-\left(1 + K\frac{\partial}{\partial K} + P\frac{\partial}{\partial P}\right)
%{\lambda}^{' \mathrm{I}; \spmqty{\sigma_1 & \sigma_2 \\ \sigma_4 & \sigma_3}}_{\spmqty{p & -p \\ k & -k }}
 -\frac{1}{2}\left( \zeta_k + \zeta_p \right)
{\lambda}^{' \mathrm{I}; \spmqty{\sigma_1 & \sigma_2 \\ \sigma_4 & \sigma_3}}_{\spmqty{p & -p \\ k & -k }}
\\ & - \frac{1}{4\pi} \int \frac{\dd q}{2 \pi \mu}\sum_{\beta, \alpha = 1}^{N_c}{\lambda}^{' \mathrm{I}; \spmqty{\sigma_1 & \sigma_2 \\ \beta & \alpha}}_{\spmqty{p & -p \\ q & -q}}{\lambda}^{' \mathrm{I}; \spmqty{\beta & \alpha \\ \sigma_4 & \sigma_3}}_{\spmqty{q & -q \\ k & -k }} -\frac{2 \mathsf{T}^{\sigma_1 \sigma_2}_{\sigma_4 \sigma_3}}{N_f}\mathsf{R}(k,p),
\end{aligned}
\label{eq:betapptilde}
\end{equation}
where 
\bqa
\zeta_k &=   \frac{\partial}{\partial \log \mu} \left[ \log Z^{(1)}(k) +  \log Z^{(3)}(k) \right],   \label{eq:hateta} \\
\mathsf{R}(k,p) &=\left[ 1 -  \frac{\partial}{\partial \log \mu} + \frac{\zeta_k + \zeta_p}{2}  \right]
\frac{{\mathsf{D}}( k;p)}{\sqrt{{V}_{F,k}{V}_{F,p}}}  \pmqty{0 & 1 \\ 1 & 0},
\label{eq:Requation}
\eqa
and we used $\dx  =- \frac{\partial}{\partial \log \mu}$ with $\mu = \Lambda \emell$.
$Z^{(i)}( k)$ defined through \eq{eq:RenormalizedQuantities}
is a function of both $k$ and $\mu$ 
although the argument $\mu$ is not shown explicitly.
Using the definition of ${\mathsf{D}}(k;p)$ 
given  in \eq{eq:Dqk},
we can can rewrite 
$\frac{{\mathsf{D}}( k;p)}{\sqrt{{V}_{F,k}{V}_{F,p}}}$ as
\bqa
\frac{{\mathsf{D}}(k;p)}{\sqrt{{V}_{F,k}{V}_{F,p}}}
= \frac{
 g_{k,p}^2
}
 { \sqrt{ V_{F,k} V_{F,p} } } \mu  D\left( \mu ,   k-p, (  v_k k + v_p p  )   \right),
\eqa
where $D( k_0, \vec k)$ is the boson propagator.
To the leading order in $v$,
we can ignore
$\dx g_{k,p}/g_{k,p}$, $\dx V_{F,k}/V_{F,k}$ and $\dx v_k/v_k$
as they are at most order of $w \ll 1$ in the small $v$ limit.
In this case, we use
\bqa
\left( 1 -  \frac{\partial}{\partial \log \mu} \right)  
\mu   D\left( \mu ,   k-p, (  v_k k + v_p p  )   \right)
 =
 - \mu^2 \frac{\partial}{\partial \mu} D\left( \mu ,   k-p, (  v_k k + v_p p  )   \right)
 \eqa
to obtain
\bqa
\mathsf{R}(k,p) &=& 
\frac{{g}_{k, p}^2}{\sqrt{{V}_{F,k}{V}_{F,p}}}\frac{\mu^2}{\left(\mu + c \abs{k -p} + c \abs{{v}_{k}k + {v}_{p}p}\right)^2} 
 \pmqty{0 & 1 \\ 1 & 0}
\label{eq:newRel}
\eqa
to the leading order in $v$.
Viewing \eq{eq:betapptilde}
as a quadratic polynomial of $ \lambda'$,
we can complete the square as
\begin{equation}
\begin{aligned}
\frac{\partial}{\partial\ell}{\lambda}^{' \mathrm{I}; \spmqty{\sigma_1 & \sigma_2 \\ \sigma_4 & \sigma_3}}_{\spmqty{p & -p \\ k & -k }} = &
- {\lambda}^{' \mathrm{I}; \spmqty{\sigma_1 & \sigma_2 \\ \sigma_4 & \sigma_3}}_{\spmqty{p & -p \\ k & -k }} 
% -\left(1 + K\frac{\partial}{\partial K} + P\frac{\partial}{\partial P} \right){\lambda}^{' \mathrm{I}; \spmqty{\sigma_1 & \sigma_2 \\ \sigma_4 & \sigma_3}}_{\spmqty{p & -p \\ k & -k }} \\ & 
\\ & -\sum_{\beta, \alpha = 1}^{N_c}\int \frac{\dd q}{2\pi\mu}\left( \frac{1}{2\sqrt{\pi}}{\lambda}^{' \mathrm{I}; \spmqty{\sigma_1 & \sigma_2 \\ \beta & \alpha}}_{\spmqty{p & -p \\ q & -q}} + 2\sqrt{\pi}{\eta}_{\beta \sigma_1 ; \alpha \sigma_2}(p, q) \right)\left( \frac{1}{2\sqrt{\pi}}{\lambda}^{' \mathrm{I}; \spmqty{\beta & \alpha \\ \sigma_4 & \sigma_3}}_{\spmqty{q & -q \\ k & -k }} + 2\sqrt{\pi}{\eta}_{\beta \sigma_4 ; \alpha \sigma_3}(q,k) \right)
\\ &  + \sum_{\beta, \alpha = 1}^{N_c}\int \frac{\dd q}{2\pi\mu} 4\pi{\eta}_{\beta \sigma_1 ; \alpha \sigma_2}(p, q){\eta}_{\beta \sigma_4 ; \alpha \sigma_3}(q,k) -\frac{2 \mathsf{T}^{\sigma_1 \sigma_2}_{\sigma_4 \sigma_3}}{N_f}\mathsf{R}(k,p),
\end{aligned}
\label{eq:etabeta}
\end{equation}
where
\begin{equation}
{\eta}_{\beta \gamma ; \alpha \delta} (k_1,k_2) = \pi \mu 
 \zeta_{k_1} 
%\left( \frac{\dd\log Z^{(1)}(K_1)}{\dd\log\mu} + \frac{\dd\log Z^{(3)}(K_1)}{\dd\log\mu}\right)
\delta(k_1 - k_2)\delta_{\beta \gamma}\delta_{\alpha \delta} I.
%\spmqty{1 & 0 \\ 0 & 1}.
\label{eq:etamatrix2}
\end{equation}
Because
$ \left|  \frac{\partial}{\partial \log \mu} \log Z^{(1)}(k) \right| 
\gg 
\left|  \frac{\partial}{\partial \log \mu}  \log Z^{(3)}(k) \right|$
in the small $v$ limit,
\bqa
\zeta_k &=&   \frac{\partial}{\partial \log \mu}   Z^{(1)}(k)  
= \frac{{g}_{k}^2(N_c^2 -1)}{\pi^2 c N_c N_f}\frac{\mu}{\mu + 2 c {v}_{k} \abs{k}}
\eqa
to the leading order in $v$,
which implies
\begin{equation}
\begin{aligned}
{\eta}_{\sigma_4 \sigma_1; \sigma_3 \sigma_2}(k_1,k_2) = & \pi \mu \frac{({g}_{k_1})^2(N_c^2 -1)}{\pi^2 c N_c N_f}\frac{\mu}{\mu + 2 c {v}_{k_1} \abs{k_1}} \delta_{\sigma_4 \sigma_1}\delta_{\sigma_3 \sigma_2}\delta(k_1-k_2) I
%\spmqty{1 & 0 \\ 0 & 1}
\\ = & 2\pi \mu \frac{\mu}{\mu + 2 c {v}_{k_1} \abs{k_1}} w^{(\eta)}_{\sigma_4 \sigma_1; \sigma_3 \sigma_2}(k_1,k_2)\delta(k_1-k_2) I,
%\spmqty{1 & 0 \\ 0 & 1},
\end{aligned}
\end{equation}
where
\begin{equation}
w^{(\eta)}_{\sigma_4 \sigma_1; \sigma_3 \sigma_2}(k_1, k_2) = \frac{\left(N_c^2 - 1\right) {g}_{k_1}^2}{2\pi^2 c N_c N_f}\delta_{\sigma_4 \sigma_1}\delta_{\sigma_3 \sigma_2}
\end{equation}
is the weight of the ${\eta}$-term.
Finally, the beta functional is obtained to be 
\begin{equation}
\begin{aligned}
\frac{\partial}{\partial\ell}{\lambda}^{' \mathrm{I}; \spmqty{\sigma_1 & \sigma_2 \\ \sigma_4 & \sigma_3}}_{\spmqty{p & -p \\ k & -k }} = & 
- {\lambda}^{' \mathrm{I}; \spmqty{\sigma_1 & \sigma_2 \\ \sigma_4 & \sigma_3}}_{\spmqty{p & -p \\ k & -k }} 
%-\left(1 + K\frac{\partial}{\partial K} + P\frac{\partial}{\partial P} \right){\lambda}^{' \mathrm{I}; \spmqty{\sigma_1 & \sigma_2 \\ \sigma_4 & \sigma_3}}_{\spmqty{p & -p \\ k & -k }} 
\\ & -\sum_{\beta, \alpha = 1}^{N_c}\int \frac{\dd q}{2\pi\mu}\left( \frac{1}{2\sqrt{\pi}}{\lambda}^{' \mathrm{I}; \spmqty{\sigma_1 & \sigma_2 \\ \beta & \alpha}}_{\spmqty{p & -p \\ q & -q}} + 2\sqrt{\pi}{\eta}_{\beta \sigma_1 ; \alpha \sigma_2}(p, q) \right)\left( \frac{1}{2\sqrt{\pi}}{\lambda}^{' \mathrm{I}; \spmqty{\beta & \alpha \\ \sigma_4 & \sigma_3}}_{\spmqty{q & -q \\ k & -k }} + 2\sqrt{\pi}{\eta}_{\beta \sigma_4 ; \alpha \sigma_3}(q,k) \right)
\\ &  + 2 \mu \left[\frac{\mu}{\mu + 2 c {v}_{k} \abs{k}}\right]^2 \frac{\left(N_c^2 - 1\right)^2 {g}_{k}^4}{\pi^2 c^2 N_c^2 N_f^2}\delta_{\sigma_4 \sigma_1}\delta_{\sigma_3 \sigma_2} \delta(p-k) I
%\spmqty{1 & 0 \\ 0 & 1} 
-\frac{2 \mathsf{T}^{\sigma_1 \sigma_2}_{\sigma_4 \sigma_3}}{N_f}\mathsf{R}(k,p).
\end{aligned}
\label{eq:etabeta2}
\end{equation}

%\end{document}
