# Supplementary material for: Field-theoretic functional renormalization group formalism for non-Fermi liquids and its application to the antiferromagnetic quantum critical metal in two dimensions
Source: arXiv:2208.00730 source file (2023-01-06)
Supplement: Supplementary file 2 [file appendixSP.tex]

\section{Flow of Single-Particle Couplings under RG}\label{appendixA_SingleParticle}
In this section we provide a full derivation both of the flow of the couplings
and the form of the crossover energy scales. 
We will first start by analyzing the general beta functions for $v_k(\ell)$,
$V_{F,k}(\ell)$, $g_{k,k'}(\ell)$ and dicuss the implications of the adiabatic
approximation to the solution of the beta functions. This discussion will lead
to a notion of diagonal couplings and an off-diagonal Yukawa coupling. From this
discussion it will also be clear that to obtain the flow of the couplings, we 
will first have to solve for the flow of the diagonal couplings, and use this to
solve for the flow of the off-diagonal Yukawa coupling.
Next, we will solve for the flow of the diagonal couplings and obtain the
crossover energy scales $E_1(k)$ and $E_2(k)$.
Finally, we will solve for the flow of the off-diagonal Yukawa coupling.  From
the final discussion we will also be able to show self-consistently that the
adiabatic condition does indeed hold to the lowest energies.

\subsection{General Discussion of Beta Function; Diagonal and Off-Diagonal Couplings} \label{appendixGeneralDecomposition}
In terms of the multiplicative counterterms, the beta functions for $\widehat
v_k(\ell)$, $\widehat V_{F,k}(\ell)$, and $\widehat g_{k,k'}(\ell)$, take the
form (cf. thesis ({\color{blue}L.13}) -- ({\color{blue}L.15})):
\begin{align}
\FR{\di v_k(\ell)}{\di\ell}     &= \FR{v_k(\ell)}{z(\ell)}     \left( \FR{\dd Z^{(2)}(k)}{\dd \log \mu} - \FR{\dd Z^{(3)}(k)}{\dd\log\mu} \right)\\
\FR{\di V_{F,k}(\ell)}{\di\ell} &= \FR{V_{F,k}(\ell)}{z(\ell)}   \left( \FR{\dd Z^{(3)}(k)}{\dd \log \mu} - \FR{\dd Z^{(1)}(k)}{\dd\log\mu} - \FR{\dd Z_{3}}{\dd\log\mu} + \FR{\dd Z_{1}}{\dd\log\mu}\right)\\
\FR{\di g_{k,k}(\ell)}{\di\ell} &= \FR{g_{k,k'}(\ell)}{z(\ell)}  \left( \left[ -\FR{\dd Z_{4}}{\dd\log\mu} +\FR{\dd Z_{1}}{\dd \log \mu} +\FR{1}{2}\FR{\dd Z_{2}}{\dd \log \mu} - \FR{1}{2}\FR{\dd Z_{3}}{\dd\log\mu} \right] 
\right.\nonumber\\
&\hspace{1.5cm}\left.
+\FR{\dd Z^{(4)}(k,k')}{\dd \log \mu} -\FR{1}{2}\FR{\dd Z^{(1)}(k)}{\dd \log \mu} - \FR{1}{2}\FR{\dd Z^{(1)}(k')}{\dd\log\mu} \right)
\end{align}

\noindent Substituting the expressions for the multiplicative counterterms (cf.
Appendix Quantum Corrections) into the above definitions we get:
\begin{align}
\FR{\di v_k(\ell)}{\di\ell}    &= \FR{v_k(\ell)}{z(\ell)}   \left( 
-\FR{4(N_c^2-1)}{\pi^3N_cN_f}\FR{g_{k,k}(\ell)^2}{V_{F,k}(\ell)}\log\PFR{V_{F,k}(\ell)}{c(\ell)}\Theta(\ell^{(2)}_k-\ell) 
\right.\nonumber\\
&\hspace{1.5cm}\left.
- \FR{2(N_c^2-1)}{\pi^4N_c^2N_f^2}
\FR{g_{k,k}(\ell)^4}{c(\ell)^2V_{F,k}(\ell)^2}\log^2\PFR{V_{F,k}(\ell)c(\ell)}{v_k(\ell)}\Theta(\ell^{(1)}_k-\ell)\right)\label{betaVgen1}\\
\FR{\di V_{F,k}(\ell)}{\di\ell}  &= \FR{V_{F,k}(\ell)}{z(\ell)}   \left( 
+\FR{2(N_c^2-1)}{\pi^3N_cN_f}\FR{g_{k,k}(\ell)^2}{V_{F,k}(\ell)}\log\PFR{V_{F,k}(\ell)}{c(\ell)}\Theta(\ell^{(2)}_k - \ell)
-\FR{N_c^2-1}{\pi^2N_cN_f}\FR{g_{k,k}(\ell)^2}{c(\ell)V_{F,k}(\ell)}\Theta(\ell^{(2)}_k-\ell)
\right.\nonumber\\
&\hspace{1.5cm}\left.
-\FR{N_c^2-1}{\pi^2N_cN_f}v_0(\ell)\log\PFR{1}{c(\ell)}
%-\FR{N_c^2-1}{8\pi^2N_c^2N_f^2}w^2\log^2\PFR{1}{w}
+\FR{N_c^2-1}{2\pi N_cN_F}w_0(\ell)
\right)\label{betaVfgen1}\\
\FR{\di g_{k,k'}(\ell)}{\di\ell} &= \FR{g_{k,k'}}{z(\ell)}\left( 
\left[
-\FR{1}{2\pi N_cN_f}w_0(\ell)\log\PFR{1}{w_0(\ell)}
+\FR{N_c^2-1}{2\pi N_cN_f}w_0(\ell)
-\FR{N_c^2-1}{\pi^2N_cN_f}v_0(\ell)\log\PFR{1}{c(\ell)}
-\FR{N_c^2-1}{8\pi^2N_c^2N_f^2}w_0^2\log^2\PFR{1}{w_0(\ell)}
\right]
\right.\nonumber\\
&\hspace{1.5cm}\left.
		+\FR{2g_{k,k}(\ell)g_{k',k'}(\ell)}{\pi^2N_cN_f(V_{F,k}(\ell)+V_{F,k'})c(\ell)}\log\PFR{(V_{F,k}(\ell)^{-1}+V_{F,k'}(\ell)^{-1})c(\ell)}{v_k(\ell)+v_{k'}(\ell)}\Theta(\ell^{(3)}_{k,k'}-\ell)
\right.\nonumber\\
&\hspace{1.5cm}\left.
-\FR{(N_c^2-1)g_{k,k}(\ell)^2    \Theta(\ell^{(2)}_{k }-\ell)  }{2\pi^2N_cN_fc(\ell)V_{F,k}(\ell) }
-\FR{(N_c^2-1)g_{k',k'}(\ell)^2 \Theta(\ell^{(2)}_{k'}-\ell) }{2\pi^2N_cN_fc(\ell)V_{F,k'}(\ell)}
\right.\nonumber\\
&\hspace{1.5cm}\left.
		-\FR{(N_c^2-1)}{4\pi^4N_c^2N_f^2}\FR{g_{k,k}(\ell)^4}{c(\ell)^2V_{F,k}(\ell)^2}\log^2\PFR{v_{k}(\ell)}{c(\ell)V_{F,k}(\ell)}\Theta(\ell^{(1)}_{k }-\ell)
\right.\nonumber\\
&\hspace{1.5cm}\left.
	%%%%
		-\FR{(N_c^2-1)}{4\pi^4N_c^2N_f^2}\FR{g_{k',k'}(\ell)^4}{c(\ell)^2V_{F,k'}(\ell)^2}\log^2\PFR{v_{k'}(\ell)}{c(\ell)V_{F,k'}(\ell)}\Theta(\ell^{(1)}_{k'}-\ell)
\right)\label{betaGgen1}
\end{align}

\noindent Let us explain the notation in the above beta functions.
The couplings have the following definitions 
$v_k(\ell) = \widehat v(k;\ell)$, 
$V_{F,k}(\ell) = \widehat V_F(k;\ell)$, and 
$g_{k,k'}(\ell) = \widehat g(k,k';\ell)$.
The notation $\widehat v(k;\ell)$ denotes $v(k(\ell);\ell)$, and similarly for the other couplings.
From the computations of the quantum corrections we
know that there are three crossover length scales that may qualitatively change
the flow of the couplings. These length scales we denote by $\ellonek,\elltwok$
and $\ellthreekkp$. The full definitions of these crossover scales are:
\begin{align}
		\label{appEnCross1}	E_1(k) \equiv \Lambda_f e^{-\ellonek} &= 2 V_{F,k}(\ellonek) v_k(\ellonek) k\\
		\label{appEnCross2}	E_2(k) \equiv \Lambda_f e^{-\elltwok} &= 2 v_k(\elltwok) c(\elltwok) k\\
		\label{appEnCross3}	E_3(k,k') \equiv \Lambda_f e^{-\ellthreekkp} &= 
		\max\left(
				2\FR{|v_k(\ellthreekkp)k+v_{k'}(\ellthreekkp)k'|}{V_{F,k}^{-1}+V_{F,k'}^{-1}},
				2v_k(\ellthreekkp)c(\ellthreekkp) k,
				2v_{k'}(\ellthreekkp)c(\ellthreekkp) k'
		\right)
\end{align}

\noindent To find expressions for the crossover length scales one should have
explicit expressions for the functional forms of $v_k,V_{F,k},g_{k,k'}$. Since
the couplings themselves depend on the crossover length scales, it follows that
one must solve for the flow of the couplings in
\cref{betaVgen1,betaVfgen1,betaGgen1} at the same time as
\cref{appEnCross1,appEnCross2,appEnCross3}.
Indeed, this is the approach that we will take below.

Before we begin solving for the flow of the couplings and the crossover length
scales, it is convenient to make one important observation, that $E_3(k,k) =
E_1(k)$ and as a result $\ellthreekk=\ellonek$ (for a proof please see the
beginning of \cref{appendixOffDiagonalFlow}).  Given this, we may notice that
when $k=k'$, \cref{betaVgen1,betaVfgen1,betaGgen1} reduces to a coupled set of
differential equations that is, most importantly, closed. In other words,
$\{v_k(\ell), V_{F,k}(\ell), g_{k,k}(\ell)\}$ is closed under the RG.  For the
remainder of the appendix we shall call this triple --- ``diagonal couplings.''
The flow of this closed set of couplings will be derived in
\cref{appendixDiagonalFlow}. Now, let us suppose that we have an explicit
solution to the diagonal couplings. By inspection of \cref{betaGgen1} it follows
that we may immediately integrate to solve for the flow of the ``off-diagonal
Yukawa coupling'' --- $g_{k,k'}(\ell)$.

\subsection{Flow of Diagonal Couplings} \label{appendixDiagonalFlow}

In this section we will solve for the flow of the couplings $\{v_k(\ell),
V_{F,k}(\ell), g_{k,k}(\ell)\}$ and find expressions for the crossover length
scales $\ellonek$ and $\elltwok$. First, let us explicitly write the form of the
IR beta functions for this set of couplings.
\begin{align}
\FR{\di v_k(\ell)}{\di\ell}    &= \FR{v_k(\ell)}{z(\ell)}   \left( 
-\FR{4(N_c^2-1)}{\pi^3N_cN_f}\FR{g_{k,k}(\ell)^2}{V_{F,k}(\ell)}\log\PFR{V_{F,k}(\ell)}{c(\ell)}\Theta(\elltwok-\ell) 
\right.\nonumber\\
&\hspace{1.5cm}\left.
- \FR{2(N_c^2-1)}{\pi^4N_c^2N_f^2}
\FR{g_{k,k}(\ell)^4}{c(\ell)^2V_{F,k}(\ell)^2}\log^2\PFR{V_{F,k}(\ell)c(\ell)}{v_k(\ell)}\Theta(\ellonek-\ell)\right)\label{betaVK}\\
\FR{\di V_{F,k}(\ell)}{\di\ell}  &= \FR{V_{F,k}(\ell)}{z(\ell)}   \left( 
+\FR{2(N_c^2-1)}{\pi^3N_cN_f}\FR{g_{k,k}(\ell)^2}{V_{F,k}(\ell)}\log\PFR{V_{F,k}(\ell)}{c(\ell)}\Theta(\elltwok - \ell)
-\FR{N_c^2-1}{\pi^2N_cN_f}\FR{g_{k,k}(\ell)^2}{c(\ell)V_{F,k}(\ell)}\Theta(\elltwok-\ell)
\right.\nonumber\\
&\hspace{1.5cm}\left.
-\FR{N_c^2-1}{\pi^2N_cN_f}v_0(\ell)\log\PFR{1}{c(\ell)}
%-\FR{N_c^2-1}{8\pi^2N_c^2N_f^2}w^2\log^2\PFR{1}{w}
+\FR{N_c^2-1}{2\pi N_cN_F}w_0(\ell)
\right)\label{betaVFK}\\
\FR{\di g_{k,k}(\ell)}{\di\ell} &= \FR{g_{k,k}}{z(\ell)}\left( 
\left[
-\FR{1}{2\pi N_cN_f}w_0(\ell)\log\PFR{1}{w_0(\ell)}
+\FR{N_c^2-1}{2\pi N_cN_f}w_0(\ell)
-\FR{N_c^2-1}{\pi^2N_cN_f}v_0(\ell)\log\PFR{1}{c(\ell)}
-\FR{N_c^2-1}{8\pi^2N_c^2N_f^2}w_0^2\log^2\PFR{1}{w_0(\ell)}
\right]
\right.\nonumber\\
&\hspace{1.5cm}\left.
+\FR{g_{k,k}(\ell)^2}{\pi^2N_cN_fV_{F,k}(\ell)c(\ell)}\log\PFR{c(\ell)}{V_{F,k}(\ell)v_k(\ell)}\Theta(\ellonek-\ell)
-\FR{(N_c^2-1)g_{k,k}(\ell)^2    \Theta(\elltwok-\ell)  }{\pi^2N_cN_fc(\ell)V_{F,k}(\ell) }
\right.\nonumber\\
&\hspace{1.5cm}\left.
		-\FR{(N_c^2-1)}{2\pi^4N_c^2N_f^2}\FR{g_{k,k}(\ell)^4}{c(\ell)^2V_{F,k}(\ell)^2}\log^2\PFR{v_{k}(\ell)}{c(\ell)V_{F,k}(\ell)}\Theta(\ellonek-\ell)
	%%%%
\right)\label{betaGKK}
\end{align}

\noindent
Before we can analyze the form of the above solutions we must have an idea about
the relation between $\ellonek$ and $\elltwok$. In view of this let us present a
proof that $\ellonek \le \elltwok$ or equivalently that $E_1(k) \ge E_2(k)$.

\vspace{.3cm}
\textbf{Theorem 1.} $E_1(k) \ge E_2(k)$.
\vspace{.3cm}

\newcommand{\mcS}{\mathcal{S}}
\noindent
\emph{Proof.} Let us look at the sets $\mcS_1$ and $\mcS_2$ defined by:
\begin{align}
\mcS_i &= \Bigl\{ (k,E_i(k)); \; k \ge 0 \Bigr\}; \;\; i=1,2.
\end{align}
The statement that $E_1(k) \ge E_2(k)$ can be reformulated graphically as the
curve $\mcS_1$ lies above $\mcS_2$, or for any $E$ if we can find $k_1,k_2$ such
that $E = E_1(k_1) = E_2(k_2)$ then $k_1 \le k_2$. Let us now express $\mcS_i$
in a way that makes the second statement manifest.  Using the definitions of
$E_1(k)$ and $E_2(k)$ in \cref{appEnCross1,appEnCross2}:
\begin{align}
\mcS_1 &= \Bigl\{ (\Lambda_f e^{-\ellonek}/2v_k(\ellonek),\Lambda_f e^{-\ellonek}); \; \ellonek \ge 0 \Bigr\}
\label{e36}
	   \\
\mcS_2 &= \Bigl\{ (\Lambda_f e^{-\elltwok}/2v_k(\elltwok)c(\elltwok),\Lambda_f e^{-\elltwok}); \; \elltwok \ge 0 \Bigr\}
\label{e37}
\end{align}
If there exists $k_1$ and $k_2$ such that $E = E_1(k_1) = E_2(k_2)$ then
using \eqref{e36} and \eqref{e37} we immediately get $\ell_* = \ell^{(1)}_{k_1} =
\ell^{(2)}_{k_2}$. We can also solve for $k_1,k_2$:
\begin{align}
		k_1 &= \Lambda_f e^{-\ell_*}/2v_k(\ell_*)&
		k_2 &= \Lambda_f e^{-\ell_*}/2v_k(\ell_*)c(\ell_*)
\end{align}
Therefore we immediately get that $k_2/k_1 = 1/c(\ell_*) \ge \sqrt{\ell_0} \ge
1$. Therefore $k_1 \le k_2$ and, as was noted earlier, this suffices to
show that $E_1(k) \ge E_2(k)$ for any fixed $k$.

\vspace{.3cm}

Now that we have the result that $\ellonek \le \elltwok$ we may start to analyze
the solution to \cref{betaVK,betaVFK,betaGKK} in three different regimes:
$0 \le \ell \le \ellonek$, $\ellonek \le \ell \le \elltwok$, $\ell \ge \elltwok$.
We will respectively call these regimes the high energy, intermediate energy,
and low energy regime.

\subsubsection{High Energy Regime}
For $0 \le \ell \le \ellonek$, the beta functions take the form 
\begin{align}
\FR{\di v_k(\ell)}{\di\ell}    &= \FR{v_k(\ell)}{z(\ell)}   \left( 
-\FR{4(N_c^2-1)}{\pi^3N_cN_f}\FR{g_{k,k}(\ell)^2}{V_{F,k}(\ell)}\log\PFR{V_{F,k}(\ell)}{c(\ell)}
- \FR{2(N_c^2-1)}{\pi^4N_c^2N_f^2}
\FR{g_{k,k}(\ell)^4}{c(\ell)^2V_{F,k}(\ell)^2}\log^2\PFR{V_{F,k}(\ell)c(\ell)}{v_k(\ell)}\right)\label{betaVKhi}\\
\FR{\di V_{F,k}(\ell)}{\di\ell}  &= \FR{V_{F,k}(\ell)}{z(\ell)}   \left( 
+\FR{2(N_c^2-1)}{\pi^3N_cN_f}\FR{g_{k,k}(\ell)^2}{V_{F,k}(\ell)}\log\PFR{V_{F,k}(\ell)}{c(\ell)}
-\FR{N_c^2-1}{\pi^2N_cN_f}\FR{g_{k,k}(\ell)^2}{c(\ell)V_{F,k}(\ell)}
\right.\nonumber\\
&\hspace{1.5cm}\left.
-\FR{N_c^2-1}{\pi^2N_cN_f}v_0(\ell)\log\PFR{1}{c(\ell)}
%-\FR{N_c^2-1}{8\pi^2N_c^2N_f^2}w^2\log^2\PFR{1}{w}
+\FR{N_c^2-1}{2\pi N_cN_F}w_0(\ell)
\right)\label{betaVFKhi}\\
\FR{\di g_{k,k}(\ell)}{\di\ell} &= \FR{g_{k,k}}{z(\ell)}\left( 
\left[
-\FR{1}{2\pi N_cN_f}w_0(\ell)\log\PFR{1}{w_0(\ell)}
+\FR{N_c^2-1}{2\pi N_cN_f}w_0(\ell)
-\FR{N_c^2-1}{\pi^2N_cN_f}v_0(\ell)\log\PFR{1}{c(\ell)}
-\FR{N_c^2-1}{8\pi^2N_c^2N_f^2}w_0^2\log^2\PFR{1}{w_0(\ell)}
\right]
\right.\nonumber\\
&\hspace{1.5cm}\left.
+\FR{g_{k,k}(\ell)^2}{\pi^2N_cN_fV_{F,k}(\ell)c(\ell)}\log\PFR{c(\ell)}{V_{F,k}(\ell)v_k(\ell)}
-\FR{(N_c^2-1)g_{k,k}(\ell)^2      }{\pi^2N_cN_fc(\ell)V_{F,k}(\ell) }
\right.\nonumber\\
&\hspace{1.5cm}\left.
-\FR{(N_c^2-1)}{2\pi^4N_c^2N_f^2}\FR{g_{k,k}(\ell)^4}{c(\ell)^2V_{F,k}(\ell)^2}\log^2\PFR{v_{k}(\ell)}{c(\ell)V_{F,k}(\ell)}	%%%%
\right)\label{betaGKKhi}
\end{align}
If we assume the initial conditions $v_k(0) = v_0(0)$, $V_{F,k}(0) = V_{F,0}(0)$
and $g_{k,k}(0) = g_{0,0}(0)$ for all $k$, then the
\cref{betaVKhi,betaVFKhi,betaGKKhi} reduce to the beta functions at the hot
spot. To see this, one can substitute the initial conditions of $v_k, V_{F,k}$,
and $g_{k,k}$ into \cref{betaVKhi,betaVFKhi,betaGKKhi} and use the identity 
$w^2\log^2 w = 4N_cN_F v\log(1/c)$. This will show that at $\ell=0$,
$\beta^{(v)}_k/v_k = 2\beta^{(g)}_{k,k}/g_{k,k}$, just as we have at the hot
spot. Since the initial condition agrees with the hot spot condition and the
differential equation that governs the flow of the couplings have the same form
as at the hot spot, this means the flow will also be the same.
The solution of \cref{betaVKhi,betaVFKhi,betaGKKhi} is then given by the flow at
the hot spot until the first crossover length scale $\ellonek$, where the beta
function changes their form. The solutions are:
\begin{align}
		\label{appHiEnSoln1}v_k^{\tra}(\ell)    \equiv v_k(0\le\ell\le\ellonek)    &= \FR{\pi^2 N_c N_f}{2(N_c^2-1)} \FR{1}{(\ell+\ell_0)\log(\ell+\ell_0)}\\
		\label{appHiEnSoln2}g_{kk}^{\tra}(\ell) \equiv g_{kk}(0\le\ell\le\ellonek) &= \sqrt{\FR{\pi^3 N_c N_f}{4(N_c^2-1)} \FR{1}{(\ell+\ell_0)\log(\ell+\ell_0)}}\\
		\label{appHiEnSoln3}V_{Fk}^{\tra}(\ell) \equiv V_{Fk}(0\le\ell\le\ellonek) &= 1
\end{align}

\subsubsection{First Crossover Scale}
Using the functional forms given in
\cref{appHiEnSoln1,appHiEnSoln2,appHiEnSoln3} we can solve to find an
expression for $\ellonek$ or equivalently $E_1(k)$. Substituting the form of
\cref{appHiEnSoln1,appHiEnSoln3} into \cref{appEnCross1}:
\begin{align}
		E_1(k) = 2 \left[ \FR{\pi^2 N_c N_f}{2(N_c^2-1)} \FR{1}{\left(\log\FR{\Lambda_f}{E_1(k)}+\ell_0)\right)
		\log\left(\log\FR{\Lambda_f}{E_1(k)}+\ell_0)\right)}\right]k
\end{align}
We shall solve this equation in two regimes:
({\color{red} $i$})  $k \gg \Lambda_f e^{-1/v_0}$, 
({\color{red} $ii$}) $k \ll \Lambda_f e^{-1/v_0}$.

\begin{list}{}{}{}

\item[({\color{red} $i$})]   First consider the momentum regime $k \gg \Lambda_f e^{-1/v_0} \sim \Lambda_f
		e^{-\ell_0}$. In order to solve for $E_1(k)$ in this regime, let us postulate the ansatz 
		\begin{align}\log(\Lambda_f/E_1(k)) \ll \ell_0\label{ansatz1}\end{align}
		which we will check self-consistently. Using this ansatz, to leading order in
		$\log(\Lambda_f/E_1(k))/\ell_0$ we get:
		\begin{align}
				E_1(k) &= 2\left[v_0(0)\left(1+\FR{\log\FR{\Lambda_f}{E_1(k)}}{\ell_0}\right)\right]k
		\end{align}
		Iteratively substituting this equation into itself we get:
		\begin{align}
				E_1(k) &=       2\left[v_0(0)\left(1+\FR{\log\FR{\Lambda_f}{2v_0(0)k}}{\ell_0}-\FR{\log\left(1+\FR{\log\FR{\Lambda_f}{E_1(k)}}{\ell_0}\right)}{\ell_0}\right)\right]k
					\\ &\approx 2\left[v_0(0)\left(1+\FR{\log\FR{\Lambda_f}{2v_0(0)k}}{\ell_0}-\FR{\log\FR{\Lambda_f}{E_1(k)}}{\ell_0^2}\right)\right]k
		\end{align}
		From here we immediately see that get the leading order solution and the leading order correction:
		\begin{align}
				E_1(k) &= 2v_0(0)k\left(1+\FR{\log\FR{\Lambda_f}{2v_0(0)k}}{\ell_0}\right)
				\label{eqn165}
		\end{align}
		We see that this solution is consistent with the ansatz \eqref{ansatz1} and within the regime $k \gg \Lambda_f e^{-1/v_0}$
		\begin{align}
				\log\FR{\Lambda_f}{2v_0(0)k} &=  \log\FR{1}{2v_0}+\log\FR{\Lambda_f}{k} \\
											 &\ll \log\FR{1}{2v_0}+\FR{1}{v_0}\\
											 &\sim \ell_0+\log\ell_0
											 \label{eqn168}
		\end{align}

\item[({\color{red} $ii$})]
		Now, let's consider the momentum regime $k \ll \Lambda_f e^{-1/v_0}$. We shall assume (and check
		self-consistently) the assumption that $\log(\Lambda_f/E_1(k)) \gg \ell_0$.
		The defining equation for $E_1(k)$ to leading order in $\ell_0/\log(\Lambda_f/E_1(k))$ becomes:
		\begin{align}
				E_1(k) = 2\left[\FR{\pi^2 N_c N_f}{2(N_c^2-1)}
				\FR{1}{\log\FR{\Lambda_f}{E_1(k)}\log\log\FR{\Lambda_f}{E_1(k)}}
				\left( 1+\FR{\ell_0}{\log\FR{\Lambda_f}{E_1(k)}} \right)
		\right] k
				\label{e169}
		\end{align}
		The solution is then:
		\begin{align}
				E_1(k) = 2\left[\FR{\pi^2 N_c N_f}{2(N_c^2-1)}
				\FR{1}{\log\FR{\Lambda_f}{k}\log\log\FR{\Lambda_f}{k}}
				\left( 1+\FR{\ell_0}{\log\FR{\Lambda_f}{k}} \right)
		\right] k
		\label{eqn170}
		\end{align}
\end{list}

\noindent
Combining \cref{eqn165,eqn170} we get the form of $E_1(k)$ for large and small
$k$:
\begin{align}
				E_1(k) &=
				\begin{cases}
				2v_0(0)k\left(1+\FR{\log\FR{\Lambda_f}{2v_0(0)k}}{\ell_0}\right)
				& k \gg \Lambda_f e^{-1/\ell_0}
				\\
				2\left[\FR{\pi^2 N_c N_f}{2(N_c^2-1)}
				\FR{1}{\log\FR{\Lambda_f}{k}\log\log\FR{\Lambda_f}{k}}
				\left( 1+\FR{\ell_0}{\log\FR{\Lambda_f}{k}} \right)
				\right] k
				& k \ll \Lambda_f e^{-1/\ell_0}
				\end{cases}
				\label{appeqn33}
\end{align}
Let us note that in \eqref{appeqn33}, the two expressions at the boundary $k =
\Lambda_f e^{-1/\ell_0}$ agree with each other. In fact, we can combine the two
expressions in \eqref{appeqn33} to obtain the simpler form:
\begin{align}
		E_1(k) &= 2v_0(\log(\Lambda_f/k))k
		\label{appeqn34}
\end{align}
Moreover, for $k \gg \Lambda_f e^{-\ell_0}$, \eqref{appeqn34} reduces to the
simple:
\begin{align}
		E_1(k) &= 2v_0(0)k
		\label{appeqn35}
\end{align}

\subsubsection{Intermediate Energy Regime}
As $\ell$ passes the first crossover length scale, $\ellonek$, the beta functions take on a new form.

\begin{align}
\widehat\beta^{(v)}_k(\ell \ge \ell^{(1)}_k) &= \FR{v_k}{z(l)}   \left( 
-\FR{4(N_c^2-1)}{\pi^3N_cN_f}\FR{g_{k,k}^2}{V_{F,k}}\log\PFR{V_{F,k}}{c}\Theta(\ell^{(2)}_k-\ell) 
\right)
\label{e171}
\\
\widehat\beta^{(V_F)}_k(\ell \ge \ell^{(1)}_k) &= \FR{V_{F,k}}{z(l)}   \left( 
+\FR{2(N_c^2-1)}{\pi^3N_cN_f}\FR{g_{k,k}^2}{V_{F,k}}\log\PFR{V_{F,k}}{c}\Theta(\ell^{(2)}_k - \ell)
\right.\nonumber\\
&\hspace{1.5cm}\left.
-\FR{N_c^2-1}{\pi^2N_cN_f}\FR{g_{k,k}^2}{cV_{F,k}}\Theta(\ell^{(2)}_k-\ell)
-\FR{N_c^2-1}{\pi^2N_cN_f}v_0\log\PFR{1}{c}
%-\FR{N_c^2-1}{8\pi^2N_c^2N_f^2}w^2\log^2\PFR{1}{w}
+\FR{N_c^2-1}{2\pi N_cN_F}w_0
\right)
\label{e172}
\\
\widehat\beta^{(g)}_{k,k}(\ell\ge\ell^{(1)}_k) &= \FR{g_{k,k}}{z(l)}\left( 
\left[
-\FR{1}{2\pi N_cN_f}w_0\log\PFR{1}{w_0}
+\FR{N_c^2-1}{2\pi N_cN_f}w_0
-\FR{N_c^2-1}{\pi^2N_cN_f}v_0\log\PFR{1}{c}
\right.\right.\nonumber\\
&\hspace{1.5cm}\left.\left.
-\FR{N_c^2-1}{8\pi^2N_c^2N_f^2}w_0^2\log^2\PFR{1}{w_0}
\right]
-\FR{(N_c^2-1)g_{k,k}^2   \Theta(\ell^{(2)}_{k }-\ell)  }{\pi^2N_cN_fcV_{F,k }}
\right)
\label{e173}
\end{align}

We expect the following. At $\ell=\ellonek$, the largest contribution to the beta function of
$g_{k,k}$ comes from the $w_0\log w_0$ term which drives $g_{k,k}$ to smaller values.
Previously, the flow of $g_{k,k}$ was governed by terms of order $v_0\log c$ and so the initial
intermediate flow will renormalize $g_{k,k}$ to zero more quickly than in the high energy flow.
As $g_{k,k}$ renormalizes to zero, we expect, at the same time that $V_{F,k}$ will renormalize
to larger values. These two statements are self-consistent. Let us also note, that at the
boundary, $\ell=\ellonek$, the beta function for $g_{k,k}$ is discontinuous whereas the beta
function for $V_{F,k}$ is continuous. As a result we also expect that the flow of $V_{F,k}$
will lag behind the flow of $g_{k,k}$.

\newcommand{\tell}{\tilde\ell}
This small $\tilde\ell \equiv \ell-\ellonek$ analysis can be made more precise. Let us expand
for small $\tell$ the coupling functions:
\begin{align}
		v_k^{\trb}(\tell)     &= v_k^{\tra}(\ellonek)     + a_1 \tell + \mathcal O(\tell)^2\\
		V_{F,k}^{\trb}(\tell) &= V_{F,k}^{\tra}(\ellonek) + a_2 \tell + a_3 \tell^2 + \mathcal O(\tell)^3\label{e20}\\
		g_{k,k}^{\trb}(\tell) &= g_{k,k}^{\tra}(\ellonek) + a_4 \tell + \mathcal O(\tell)^2
\end{align}
In eqn.~\eqref{e20} we have anticipated that the coefficient of the linear
term, $a_2$, will vanish because at $\ell=\ellonek$ the beta function
$\widehat\beta^{(V_F)}_k(\ellonek) = 0$.
Substituting these functional forms into the beta functions will lead to the following algebraic expressions written to leading order in $\ell_0$:
\begin{align}
		a_1 &= - \FR{4(N_c^2-1)}{\pi^3 N_c N_f} v_k^{\tra}(\ellonek) g_{k,k}^{\tra}(\ellonek)^2 \log\PFR{1}{c(\ellonek)}\\
		a_2 &= 0\\
		a_3 &= - \FR{N_c^2-1}{\sqrt2 \pi^{3/2} N_cN_f}  \FR{a_4\sqrt{v_k^{\tra}(\ellonek)}}{c(\ellonek)} \\
		a_4 &= - \FR{1}{2\pi N_c N_f} g_{k,k}^{\tra}(\ellonek) w_0(\ellonek) \log \PFR{1}{w_0(\ellonek)} 
\end{align}
Let us expand the functional forms to get a more explicit expression for $a_1, a_3,$ and $a_4$:
\begin{align}
		a_1 &= - v_k^{\tra}(\ellonek) \FR{2(N_c^2-1)}{\pi^2 N_c N_f} 
		\left[
				\FR{\pi^2N_cN_f}{2(N_c^2-1)} \FR{1}{(\ellonek+\ell_0)\log(\ellonek+\ell_0)}
		\right]
		\log
		\left[
				\FR{4\sqrt{N_c^2-1}\sqrt{\ellonek+\ell_0}}{\pi}
		\right]
		\\
		a_3 &= - \FR{1}{2\pi N_c N_f} %g_{k,k}^{\tra}(\ellonek)
		\left[
				\FR{2\pi N_c N_f}{\sqrt{N_c^2-1}}\FR{1}{\sqrt{\ellonek+\ell_0}\log(\ellonek+\ell_0)}
		\right]
		\log 
		\left[
				\FR{\sqrt{N_c^2-1}}{2\pi N_c N_f}\sqrt{\ellonek+\ell_0}\log(\ellonek+\ell_0)
		\right]
		\nonumber\\&\times
		\FR{-(N_c^2-1)}{\sqrt2 \pi^{3/2} N_cN_f}  %\FR{\sqrt{v_k^{\tra}(\ellonek)}}{c(\ellonek)} 
		\sqrt{\FR{\pi}{2}}
		\left[ \FR{\pi^2 N_c N_f}{2(N_c^2-1)} \FR{1}{(\ellonek+\ell_0)\log(\ellonek+\ell_0)} \right]
		\left[\FR{4\sqrt{N_c^2-1}\sqrt{\ellonek+\ell_0}}{\pi}\right]
		\\
		a_4 &= - \FR{g_{k,k}^{\tra}(\ellonek)}{2\pi N_c N_f} 
		\left[
				\FR{2\pi N_c N_f}{\sqrt{N_c^2-1}}\FR{1}{\sqrt{\ellonek+\ell_0}\log(\ellonek+\ell_0)}
		\right]
		\log 
		\left[
				\FR{\sqrt{N_c^2-1}}{2\pi N_c N_f}\sqrt{\ellonek+\ell_0}\log(\ellonek+\ell_0)
		\right]
\end{align}
Simplifying
\begin{align}
		a_1 &= - v_k^{\tra}(\ellonek)
		\left[ \FR{1}{(\ellonek+\ell_0)\log(\ellonek+\ell_0)} \right]
		\log \left[ \FR{4\sqrt{N_c^2-1}\sqrt{\ellonek+\ell_0}}{\pi} \right]
		\\
		a_3 &=  %g_{k,k}^{\tra}(\ellonek)
		\left[  \FR{1}{(\ellonek+\ell_0)\log^{3/2}(\ellonek+\ell_0)} \right]
		\log 
		\left[
				\FR{\sqrt{N_c^2-1}}{2\pi N_c N_f}\sqrt{\ellonek+\ell_0}\log(\ellonek+\ell_0)
		\right]
		\\
		a_4 &= - \FR{g_{k,k}^{\tra}(\ellonek)}{\sqrt{N_c^2-1}} 
		\left[
				\FR{1}{\sqrt{\ellonek+\ell_0}\log(\ellonek+\ell_0)}
		\right]
		\log 
		\left[
				\FR{\sqrt{N_c^2-1}}{2\pi N_c N_f}\sqrt{\ellonek+\ell_0}\log(\ellonek+\ell_0)
		\right]
\end{align}

We shall not expand the above expressions for small $\ellonek$ because $\ellonek$ may not be
small! Nevertheless, these are the coefficients that describe the flow of $v_k$, $V_{F,k}$ and
$g_{k,k}$ to leading order in $\tell \equiv \ell-\ellonek$. Explicitly the coupling functions 
as a functions of $\tell$ are given by:
\begin{align}
		\begin{split} \label{pertFlow1}
		v_k^{\trb}(\tell+\ellonek) &= v_k^{\tra}(\ellonek)\left[ 1 - 
		\FR{\tell}{(\ellonek+\ell_0)\log(\ellonek+\ell_0)} 
		\log \left[ \FR{4\sqrt{N_c^2-1}\sqrt{\ellonek+\ell_0}}{\pi} \right]
		\right]\\
		V_{F,k}^{\trb}(\tell+\ellonek)&=\FR{\tell^2}{2(\ellonek+\ell_0)\log(\ellonek+\ell_0)}+\mathcal O(\tell)^3\\
		g_{k,k}^{\trb}(\tell+\ellonek) &= g_{k,k}^{\tra}(\ellonek)\left[ 1 -
				\FR{\tell(N_c^2-1)^{-1/2}}{\sqrt{\ellonek+\ell_0}\log(\ellonek+\ell_0)}
		\log 
		\left[
				\FR{\sqrt{N_c^2-1}}{2\pi N_c N_f}\sqrt{\ellonek+\ell_0}\log(\ellonek+\ell_0)
		\right]
\right]
		\end{split}
\end{align}

\begin{figure}[h!]
\centering
\includegraphics[scale=.4]{./may5plt1.pdf}
\includegraphics[scale=.4]{./may5plt2.pdf}
\caption{
		Left  figure: Accuracy of perturbative solution for $g_{k,k}$.
		Right figure: Accuracy of perturbative solution for $v_{k}$.
		Blue: Numerical solution of RG flow.
		Orange: Perturbative solution of $g_{k,k}^{\trb},v_k^{\trb}$.
}
\end{figure}

\begin{figure}[h!]
\centering
\includegraphics[scale=.4]{./may6plt3.pdf}
\caption{
		Accuracy of perturbative solution for $V_{F,k}$ between $\ellonek$ and $\elltwok$.
		Blue: Numerical solution of RG flow.
		Orange: Perturbative solution of $V_{F,k}^{\trb}$.
}
\end{figure}

From these expressions we immediately see the regime of validity of these solutions does not
extend further than $\tell\sim\sqrt{\ellonek+\ell_0}\sim\max(\sqrt{\ellonek},\sqrt{\ell_0})$.
At these length scales $g_{k,k}$ starts to flow much more rapidly and these perturbative
arguments break down. These perturbative arguments also show that $V_{F,k}$ flows much more
slowly than either of $g_{k,k}$ or $v_k$ in the intermediate regime \emph{at the beginning} of
this intermediate regime. If it turns out that $\elltwok-\ellonek \gg \sqrt{\ellonek+\ell_0}$
then we analyze the flow of the couplings more carefully. Using the above flow
\eqref{pertFlow1}, we may check whether or not there exists a self-consistent solution to
$\elltwok$ already in this perturbative regime.

\subsubsection{Second Crossover Scale}

The self-consistent equation for $E_2(k)$ is given by:
\begin{align}
		E_2(k) = 2v^{\trb}_k\left( \log\FR{\Lambda_f}{E_2(k)} \right) c\left( \log\FR{\Lambda_f}{E_2(k)} \right) k
		\label{implicitE2K}
\end{align}
Before we substitute the $\ell$-dependence of $v_k^{\trb}$ and $c$, let us first expand
$c(\tell+\ellonek)$ for small $\tell$.
\begin{align}
		c(\tell+\ellonek) = c(\ellonek)\left[1-\FR{\tell}{2(\ellonek+\ell_0)}\right]
\end{align}
Let us now substitute the $\ell$-dependence of the coulpings as per \eqref{pertFlow1}.  
\begin{align}
		E_2(k) = 2 v_k^{\tra}(\ellonek) c(\ellonek) k
		\left( 1 - 
				\FR{\log\FR{\Lambda_f}{E_2(k)}-\ellonek}{(\ellonek+\ell_0)\log(\ellonek+\ell_0)} 
		\log  \left[ \FR{4\sqrt{N_c^2-1}\sqrt{\ellonek+\ell_0}}{\pi} \right]
		\right)
		%\\\times
		\left(1-\FR{\log\FR{\Lambda_f}{E_2(k)}-\ellonek}{2(\ellonek+\ell_0)}\right)
		%\left[ \FR{\pi}{4\sqrt{N_c^2-1}\sqrt{\log\FR{\Lambda_f}{E_2(k)}+\ell_0}} \right]
		\label{e206}
\end{align}
%Immediately we see an interesting remark, that if $\tell \equiv \log(\Lambda_f/E_2(k))-\ellonek \ll \ellonek+\ell_0$
%then we may ignore the leading order terms and find the solution:
%\begin{align}
%		E_2(k) = 2 v_k^{\tra}(\ellonek) c(\ellonek) k
%		\label{e207}
%\end{align}

%Let us evaluate the regime of validity of the solution in \eqref{e207}. 
%Looking at \eqref{e206} we see that \eqref{e207} is valid when
The perturbative corrections in \eqref{e206} are small whenever:
\begin{align}
		{\ellonek + \ell_0} &\gg \elltwok-\ellonek = \log\FR{E_1(k)}{E_2(k)}. 
		\label{e208}
\end{align}
This gives the result:
\begin{align}
		E_2(k) = 2 v_k^{\tra}(\ellonek) c(\ellonek) k.
		\label{e207}
\end{align}
Analyzing the RHS of \eqref{e208} in view of \eqref{e207} and the solutions of $\ellonek$ found in \eqref{eqn165} and
\eqref{e169}:
\begin{align}
\log\FR{E_1(k)}{E_2(k)}
	&= 
	\begin{cases}
			\log \FR{2v_0(0) k}{2v_0(\ellonek) c(\ellonek)k} & k \gg \Lambda_f e^{-1/v_0}\\
			\log \FR{2v_0(\log(\Lambda_f/k) k}{2v_0(\ellonek) c(\ellonek)k} & k \ll \Lambda_f e^{-1/v_0}
	\end{cases}
	\label{e211a}
	\\
	&\sim - \log c(\ellonek) 
	\\
	&\sim \log(\ellonek+\ell_0) 
	\label{e211}
\end{align}
In both cases of \eqref{e211a}, the $v_0$ dependence approximately cancels out.
Indeed using \eqref{e211} we see that \eqref{e208} is always satisfied for all
momenta. The conclusion is then that $E_2(k)$ is reached well-within the
perturbative regime and so the solutions in \eqref{pertFlow1} hold for the
entire intermediate regime.

The final values, keeping only the leading order corrections, of the coupling
functions at the boundary are then given by
\begin{align}
		\begin{split}\label{finalValues}
		v_k^{\trb}(\elltwok) &= v_k^{\tra}(\ellonek)
		\left[ 1 - \FR{ \log (\ellonek+\ell_0) }{4(\ellonek+\ell_0)} \right]\\
		V_{F,k}^{\trb}(\elltwok) &= 1\\
		g_{k,k}^{\trb}(\elltwok) &= g_{k,k}^{\tra}(\ellonek)
		\left[ 1 - \FR{\log(\ellonek+\ell_0)}{4\sqrt{N_c^2-1}\sqrt{\ellonek+\ell_0}} \right]
		\end{split}
\end{align}
As we can see, to leading order we may assume that the flow is cutoff at
$\ellonek$.

\subsubsection{Low Energy Regime}

In this section I would like to write down the low energy flow.  The low-energy
regime starts at $\ell \ge \ell^{(2)}_k$. The beta functions are given by:

\begin{align}
\widehat\beta^{(v)}_k(\ell \ge \ell^{(2)}_k) &= 0\\
\widehat\beta^{(V_F)}_k(\ell \ge \ell^{(2)}_k) &= \FR{V_{F,k}}{z(l)}   \left( 
-\FR{N_c^2-1}{\pi^2N_cN_f}v_0\log\PFR{1}{c}
+\FR{N_c^2-1}{2\pi N_cN_F}w_0
\right)
\\
\widehat\beta^{(g)}_{k,k}(\ell\ge\ell^{(2)}_k) &= \FR{g_{k,k}}{z(l)}\left( 
-\FR{1}{2\pi N_cN_f}w_0\log\PFR{1}{w_0}
+\FR{N_c^2-1}{2\pi N_cN_f}w_0
\right.\nonumber\\
&\hspace{1cm}\left.
-\FR{N_c^2-1}{\pi^2N_cN_f}v_0\log\PFR{1}{c}
-\FR{N_c^2-1}{8\pi^2N_c^2N_f^2}w_0^2\log^2\PFR{1}{w_0}
\right)
\end{align}

\noindent 
To give an feel for the numerical size of the couplings appearing in the above
beta functions, for $\ell_0 \sim 10^5$:
\begin{align}
		v_0 &\sim \FR{1}{\ell_0\log\ell_0}\sim 0.2\times 10^{-5}
& c_0 &\sim \FR{1}{\sqrt{\ell_0}}\sim 10^{-2.5}
& w_0 &\sim \FR{1}{\sqrt{\ell_0}\log\ell_0}\sim0.2\times 10^{-2.5}
\end{align}

\noindent
From these relations it is clear that for $\ell_0\sim10^5$ the beta functions
take the form:
\begin{align}
\widehat\beta^{(v)}_k(\ell \ge \ell^{(2)}_k) &= 0\\
\widehat\beta^{(V_F)}_k(\ell \ge \ell^{(2)}_k) &= \FR{V_{F,k}}{z(l)}   \left( 
+\FR{N_c^2-1}{2\pi N_cN_F}w_0
\right)
\\
\widehat\beta^{(g)}_{k,k}(\ell\ge\ell^{(2)}_k) &= \FR{g_{k,k'}}{z(l)}\left( 
-\FR{1}{2\pi N_cN_f}w_0\log\PFR{1}{w_0}
+\FR{N_c^2-1}{2\pi N_cN_f}w_0
\right)
\end{align}

\noindent 
From here the flow of $V_{F,k}$ and $g_{kk}$ is straightforward to determine:
\begin{align}
		\begin{split}\label{appLowEnSolnFinal}
v_k(\ell) &= \FR{\pi^2 N_c N_f}{2(N_c^2-1)} \FR{1}{(\ell^{(1)}_k+\ell_0)\log(\ell^{(1)}_k+\ell_0)} 
		\left[ 1 - \FR{ \log (\ellonek+\ell_0) }{4(\ellonek+\ell_0)} \right]\\
%\exp\left[ + \FR{\sqrt{N^2_c-1}}{(\ell^{(1)}_k+\ell_0)\log(\ell^{(1)}_k+\ell_0)} 
%		\right.\\&\hspace{-1cm}\left.
%\times\log\PFR{4\sqrt{\ell^{(1)}_k+\ell_0}}{\pi\sqrt{N_c^2-1}} 
%\left(\sqrt{\ell^{(2)}_k+\ell_0}
%e^{-\FR{2}{\sqrt{N_c^2-1}}\left(\sqrt{\ell^{(2)}_k+\ell_0}-\sqrt{\ell^{(1)}_k+\ell_0}\right)}
%-\sqrt{\ell^{(1)}_k+\ell_0}
%\right) \right]\\
%\exp\left[ \FR{1}{2}\sqrt{\FR{N^2_c-1}{\ell^{(1)}_k+\ell_0}} \right]\\
V_{F,k}(\ell) &= \exp\left( 
\sqrt{N_c^2-1} \left[
\mathrm{Ei}\left(\FR{1}{2}\log(\ell+\ell_0)\right)-\mathrm{Ei}\left(\FR{1}{2}\log(\elltwok+\ell_0)\right)
\right]
\right)\\
g_{kk}(\ell)&= \sqrt{\FR{\pi^3 N_c N_f}{4(N_c^2-1)} \FR{1}{(\ell^{(1)}_k+\ell_0)\log(\ell^{(1)}_k+\ell_0)}} 
		\left[ 1 - \FR{\log(\ellonek+\ell_0)}{4\sqrt{N_c^2-1}\sqrt{\ellonek+\ell_0}} \right]
\\&\hspace{-1cm}\times
\exp\left(
- \FR{\sqrt{\ell+\ell_0}-\sqrt{\elltwok+\ell_0}}{\sqrt{N_c^2-1}}
+
\sqrt{N_c^2-1} \left[
\mathrm{Ei}\left(\FR{1}{2}\log(\ell+\ell_0)\right)-\mathrm{Ei}\left(\FR{1}{2}\log(\elltwok+\ell_0)\right)
\right]
\right)
\end{split}
\end{align}

In summary, the flow of the diagonal couplings for a fixed momentum $k$ is given by:
\begin{align}
\label{appSolnFinal1}
v_k(\ell) &=
		\begin{cases}
v_k^{\tra}(\ell)\equiv \FR{\pi^2 N_c N_f}{2(N_c^2-1)} \FR{1}{(\ell+\ell_0)\log(\ell+\ell_0)} & \ell \le \ellonek\\
v_k^{\trb}(\ell)\equiv v_k^{\tra}(\ellonek) \left[1-\FR{\ell-\ellonek}{(\ellonek+\ell_0)}\right] & \ellonek \le \ell \le \elltwok\\
v_k^{\trc}(\ell)\equiv v_k^{\tra}(\ellonek) \left[1-\FR{\elltwok-\ellonek}{(\ellonek+\ell_0)}\right] & \ell \ge \elltwok
		\end{cases}
\\
\label{appSolnFinal2}
V_{F,k}(\ell) &=
        	\begin{cases}
V_{F,k}^{\tra}(\ell)\equiv 1 & \ell \le \ellonek\\
V_{F,k}^{\trb}(\ell)\equiv 1 & \ellonek \le \ell \le \elltwok \\
V_{F,k}^{\trc}(\ell)\equiv \exp\left( \sqrt{N_c^2-1} \left[ \mathrm{Ei}\left(\FR{1}{2}\log(\ell+\ell_0)\right)-\mathrm{Ei}\left(\FR{1}{2}\log(\elltwok+\ell_0)\right) \right] \right) & \ell \ge \elltwok
		\end{cases}
\\
\label{appSolnFinal3}
g_{k,k}(\ell) &=
         \begin{cases}
g_{k,k}^{\tra}(\ell)\equiv \sqrt{\FR{\pi^3 N_c N_f}{4(N_c^2-1)} \FR{1}{(\ell+\ell_0)\log(\ell+\ell_0)}} & \ell \le \ellonek\\
g_{k,k}^{\trb}(\ell)\equiv g_{k,k}^{\tra}(\ellonek)\left[ 1 - \FR{\ell-\ellonek}{4\sqrt{N_c^2-1}\sqrt{\ellonek+\ell_0}} \right]  & \ellonek \le \ell \le \elltwok \\
g_{k,k}^{\trc}(\ell)\equiv g_{k,k}^{\trb}(\elltwok) 
\exp\left( - \FR{\sqrt{\ell+\ell_0}-\sqrt{\elltwok+\ell_0}}{\sqrt{N_c^2-1}} + \sqrt{N_c^2-1} \left[ \mathrm{Ei}\left(\FR{1}{2}\log(\ell+\ell_0)\right)-\mathrm{Ei}\left(\FR{1}{2}\log(\elltwok+\ell_0)\right) \right] \right) 
& \ell \ge \elltwok
         \end{cases}
\end{align}

\subsubsection{Momentum Profile of Diagonal Couplings}
In this section, let us fix the energy scale $\mu \equiv \Lambda_f e^{-\ell}$
and obtain the momentum profile of the diagonal couplings.  We will do this in
two goes for $\mu \gg \Lambda_fe^{-\ell_0}/2v_0(0)$ and for $\mu \ll
\Lambda_fe^{-\ell_0}/2v_0(0)$.

\begin{list}{}{}{}
\item[({\color{red}$i$})]
		First we assume the heirarchy: $\mu \gg \Lambda_f e^{-\ell_0}/2v_0(0)
		\sim \Lambda_F \ell_0 e^{-\ell_0}$.

Angle: $v(k;\mu)$.
\begin{align}
		\label{appA71}
		v(k;\mu)
		&= 
		\begin{cases}
				\FR{\pi^2 N_c N_f}{2(N_c^2-1)} 
				\FR{1}{(\ell_\mu+\ell_0)\log(\ell_\mu+\ell_0)} 
		& 0 \le k \le \mu/2v_0(0)\\
				v_0\left(\log\FR{\Lambda_f}{2v_0(0)|k|}\right)
				\left[1-\FR{\log(2v_0|k|/\mu)}{(\log(\Lambda_f/2v_0(0)|k|)+\ell_0)}\right]
		& \mu/2v_0(0) \le k \le \mu/2v_0(0)c(0)\\
				v_0\left(\log\FR{\Lambda_f}{2v_0(0)|k|}\right)
				\left[1-\FR{\log(1/c(0))}{(\log(\Lambda_f/2v_0(0)|k|)+\ell_0)}\right]
		& \mu/2v_0(0)c(0) \le k \le \Lambda_f/2v_0(0)\\
				v_0(0)
				\left[1-\FR{\log(\Lambda_f/2v_0(0)c_0k)}{\ell_0}\right]
		& \Lambda_f/2v_0(0) \le k \le \Lambda_f/2v_0(0)c(0)\\
				v_0(0) 
		& k \ge \Lambda_f/2v_0(0)c(0)\\
		\end{cases}
\end{align}

Fermi Velocity: $V_F(k;\mu)$.
\begin{align}
		\label{appA72}
		V_F(k;\mu)
		&= 
		\begin{cases}
				1
		& 0 \le k \le \mu/2v_0(0)c(0)\\
\exp\left( \sqrt{N_c^2-1} \left[ \mathrm{Ei}\left(\FR{1}{2}\log(\ell_\mu+\ell_0)\right)-\mathrm{Ei}\left(\FR{1}{2}\log\left(\log\FR{\Lambda_f}{2v_0(0)c(0)k}+\ell_0\right)\right) \right] \right)
		& \mu/2v_0(0)c(0) \le k \le \Lambda_f/2v_0(0)c(0)\\
\exp\left( \sqrt{N_c^2-1} \left[ \mathrm{Ei}\left(\FR{1}{2}\log(\ell_\mu+\ell_0)\right)-\mathrm{Ei}\left(\FR{1}{2}\log\ell_0\right) \right] \right)
		& k \ge \Lambda_f/2v_0(0)c(0)\\
		\end{cases}
\end{align}

Let us define two functions:
\begin{align}
\mc E_0(\ell_a,\ell_b) &\equiv \exp\left(-\FR{\sqrt{\ell_a+\ell_0}-\sqrt{\ell_b+\ell_0}}{\sqrt{N_c^2-1}}\right)\\
\mc E_1(\ell_a,\ell_b) &\equiv
\exp\left(\sqrt{N_c^2-1}\left(\mathrm{Ei}(\log\sqrt{\ell_a+\ell_0})-\mathrm{Ei}(\log\sqrt{\ell_b+\ell_0})\right)\right)
\end{align}

Diagonal Yukawa Coupling: $g(k,k;\mu)$.
\begin{align}
		\label{appA73}
		g(k,k;\mu)
		&= 
		\begin{cases}
\sqrt{\FR{\pi^3 N_c N_f}{4(N_c^2-1)}\FR{1}{(\ell_\mu+\ell_0)\log(\ell_\mu+\ell_0)}}
		& 0 \le k \le \mu/2v_0(0)\\
\sqrt{\FR\pi2 v_0\left(\log\FR{\Lambda_f}{2v_0(0)|k|}\right)}
\left[1-\FR{\log(2v_0(0)k/\mu)/4\sqrt{N_c^2-1}}{\sqrt{\log(\Lambda_f/2v_0(0)k)+\ell_0}} \right]
		& \mu/2v_0(0) \le k \le \mu/2v_0(0)c(0)\\
		\left(
\sqrt{\FR\pi2 v_0\left(\log\FR{\Lambda_f}{2v_0(0)|k|}\right)}
\left[1-\FR{\log(1/c(0))/4\sqrt{N_c^2-1}}{\sqrt{\log(\Lambda_f/2v_0(0)k)+\ell_0}} \right]
\mc E_0(\ell,\elltwok) \mc E_1(\ell,\elltwok)
		\right)
		& \mu/2v_0(0)c(0) \le k \le \Lambda_f/2v_0(0)\\
		\left(
\sqrt{\FR\pi2 v_0(0)}
\left[1-\FR{\log(\Lambda_f/2v_0(0)c_0k)/4\sqrt{N_c^2-1}}{\sqrt{\ell_0}} \right]
\mc E_0(\ell,\elltwok)
\mc E_1(\ell,\elltwok)
		\right)
		& \Lambda_f/2v_0(0) \le k \le \Lambda_f/2v_0(0)c(0)\\
		\left(
\sqrt{\FR\pi2 v_0(0)}
\mc E_0(\ell,0)
\mc E_1(\ell,0)
		\right)
		& k \ge \Lambda_f/2v_0(0)c(0)\\
		\end{cases}
		\intertext{where}
		\elltwok &\equiv \log(\Lambda_f/2v_0(0)c(0)k)
\end{align}

\item[({\color{red}$ii$})]
		Now, if we assume the heirarchy $\mu \ll \Lambda_f e^{-\ell_0}$, the
		form of \cref{appA71,appA72,appA73} does not change except for the
		crossover scales.  Instead of $\mu/v_0(0)$ we will have the momentum
		scale $k_1$ such that $E(k_1) \le \mu$; since $\mu \ll \Lambda_f
		e^{-\ell_0}$, it follows that $E_1(k)$ will take on the more complicated
		form given in \cref{appeqn33}. Similarly, $\mu/v_0(0)c(0)$ should get
		replaced with a different form so that $k \le \mu/v_0(0)c(0)$ would be
		equivalent to $E_2(k) \le \mu$ where $E_2(k)$ is given by the general
		form \cref{e207}.

\end{list}

%\cref{appSolnFinal1,appSolnFinal2,appSolnFinal3} and simply read off the solution:

\subsection{Flow of Off-Diagonal Yukawa Coupling} \label{appendixOffDiagonalFlow}

\subsubsection{Third Crossover Scale}
In this section we will first
understand the structure of $E_3(k,k')$, then we will show that
$E_3(k,k)=E_1(k)$, and finally we will compute $E_3(k,k')$ as a function of the
first and second crossover energy scales. Let us start by recalling that the
definition of $E_3(k,k')$:
\begin{align}
		\begin{split}\label{e56}
		E_3(k,k')&=\max\left(
		\FR{2|v_k(\ellthreekkp)k+v_{k'}(\ellthreekkp)k'|}{V_{F,k}(\ellthreekkp)^{-1}+V_{F,k'}(\ellthreekkp)^{-1}},
		2v_k(\ellthreekkp)c(\ellthreekkp)|k|,
		2v_k(\ellthreekkp)c(\ellthreekkp)|k'|
\right)
		\\
\ellthreekkp &= \log\PFR{\Lambda_f}{E_3(k,k')}
		\end{split}
\end{align}

\noindent 
An equivalent definition can be given as:
\begin{align}
		\begin{split}\label{e57}
				\begin{aligned}
		E_3(k,k')&=\max\left( E_3^{(0)}(k,k'), E_3^{(1)}(k), E_3^{(2)}(k') \right) \\
		E_3^{(0)}(k,k')&=\FR{2|v_k(\ellthreezerokkp)k+v_{k'}(\ellthreezerokkp)k'|}{V_{F,k}(\ellthreezerokkp)^{-1}+V_{F,k'}(\ellthreezerokkp)^{-1}} &
		\ellthreezerokkp &= \log\PFR{\Lambda_f}{E_3^{(0)}(k,k')}\\
		E_3^{(1)}(k )&= 2v_k(\ellthreeonekkp)c(\ellthreeonekkp)|k| &
		\ellthreeonekkp &= \log\PFR{\Lambda_f}{E_3^{(1)}(k )}\\
		E_3^{(2)}(k')&= 2v_{k'}(\ellthreetwokkp)c(\ellthreetwokkp)|k'| &
		\ellthreetwokkp &= \log\PFR{\Lambda_f}{E_3^{(2)}(k')}
				\end{aligned}
		\end{split}
\end{align}

\noindent To understand why \eqref{e56} is equivalent to \eqref{e57}, let us
suppose that the maximum function chooses the first argument in \eqref{e56}. In
this situation the defining equation for $E_3(k,k')$ corresponds to that of
$E_3^{(0)}(k,k')$. When the maximum function in \eqref{e56} chooses the second
argument then the defining equation is the same as $E_3^{(1)}(k)$, and similarly
for the third argument. Moreover, the defining equations for $E_3^{(1)}$ and
$E_3^{(2)}$ correspond with the defining equations for the second crossover
scale $E_2$ given in \eqref{implicitE2K}. This means that
\begin{align}
		E_3(k,k')&=\max\left( E_3^{(0)}(k,k'), E_2(k), E_2(k') \right).
		\label{e64}
\end{align}
Using this alternative form of $E_3(k,k')$, as the maximum of three independent
energy scales, we will be able to more easily understand the properties of
$E_3(k,k')$ and also be able to find an explicit form for $E_3(k,k')$.

Now let us address the observation made in \cref{appendixGeneralDecomposition}
that $E_3(k,k) = E_1(k)$. This remark was important in order to separate the
diagonal couplings from the off-diagonal Yukawa coupling and therefore be able
to simplify the solution of the beta functions. Substituting $k'=k$ in
\cref{e64} we get that $E_3(k,k) = \max(E_1(k),E_2(k))$ and using the fact that
$E_1(k) \ge E_2(k)$ (cf \cref{appendixDiagonalFlow}), we get $E_3(k,k)=E_1(k)$.

Let us now begin solve for an expression of $E_3(k,k')$ in terms of the first
and second energy crossover scales, $E_1$ and $E_2$. From \cref{e64}, there are
three cases to consider: $E_3(k,k') = E_3^{(0)}(k)$, $E_3(k,k') = E_2(k)$,
$E_3(k,k') = E_2(k')$. In the latter two cases, we may use the expression
\eqref{e206} to get an explicit expression for $E_3(k,k')$. In the first case,
the additional inequality, 
\begin{align}E_3^{(0)}(k,k') = E_3(k,k') \ge E_2(k), E_2(k'),\label{e65}\end{align} 
which is obtained directly from \eqref{e64} allows us to make some
simplifications in the solution for $E_3^{(0)}$ in the case when $E_3^{(0)} =
E_3$. When solving for $E_3^{(0)}$, the inequality \eqref{e65} allows us to
use the fact that $V_{F,k} = V_{F,k'} = 1$.
\begin{align}
		\label{e66}
		E_3^{(0)}(k,k')&=\Bigl|v_k(\ellthreezerokkp)k+v_{k'}(\ellthreezerokkp)k'\Bigr| &
		\ellthreezerokkp &= \log\PFR{\Lambda_f}{E_3^{(0)}(k,k')}
\end{align}

First let us show that $E_3^{(0)}(k,k') \le \max(E_1(k),E_1(k'))$.
Suppose the contrary that $E_3^{(0)}(k,k') > \max(E_1(k),E_1(k'))$.
This means that in the defining equation for $E_3^{(0)}$ (in the regime that we
are interested in) we may simplify the form of $v_k$ and use $v_k=v_{k'}=v_0$:
\begin{align}
E_3^{(0)}(k,k') = v_0(\ellthreezerokkp)|k+k'|
\label{e69}
\end{align}
Solving for $|k+k'|$ in terms of $\ellthreezerokkp$ we get:
\begin{align}
		|k+k'| &= \Lambda_f e^{-\ellthreezerokkp}/v_0(\ellthreezerokkp)
		\sim \Lambda_f e^{-\ellthreezerokkp}(\ellthreezerokkp+\ell_0)
\end{align}
Doing the same for $|k|,|k'|$, 
\begin{align}
		|k+k'| &\le |k| + |k'|
		\label{e71}
		\\
			   &=\Lambda_f \left( 
					   \FR{e^{-\ellonek}}{2v_0(\ellonek)} + 
					   \FR{e^{-\ellonekp}}{2v_0(\ellonekp)} 
			   \right)
			   \label{e72}
			   \\
			   &\le \Lambda_f \left( 
					   \FR{e^{-\ellthreezerokkp}}{2v_0(\ellthreezerokkp)} + 
					   \FR{e^{-\ellthreezerokkp}}{2v_0(\ellthreezerokkp)} 
			   \right)
			   \label{e73}
			   \\
			   &= |k+k'|
			   \label{e74}
\end{align}
When going from \eqref{e72} to \eqref{e73} we used our assumption that
$E_3^{(0)}(k,k') \ge E_1(k),E_1(k')$ (or equivalently $\ellthreezerokkp \le
\ellonek,\ellonekp$) and $e^{-\ell}/v_0(\ell)$ is a monotonically decreasing
function of $\ell$.
Combining \eqref{e71} and \eqref{e74} we arrive at the conclusion that $k=k'$ or
$k=-k'$. In both cases, however, we violate two of our initial assumptions: when
$k=k'$ we have $E_3^{(0)}(k,k') = E_1(k) = E_1(k')$ whereas we assumed that
$E_3^{(0)}(k,k') > E_1(k),E_1(k')$; and when $k=-k'$, we can immediately use
definition \eqref{e66} to conclude that $E_3^{(0)}(k,k')=0 \le E_1(k),E_1(k')$.
Therefore we have arrived at a contradiction showing that, under our current
assumption that $E_3(k,k') \ge E_2(k),E_2(k')$, $E_3^{(0)}(k,k')$ must satisfy
\begin{align}
		E_3^{(0)}(k,k') \le \max(E_1(k),E_1(k')).
		\label{e75}
\end{align}
The conclusion is that in fact \cref{e75} is the true relation between
$E_3^{(0)}(k,k')$, $E_1(k)$, $E_1(k')$.
Equation \eqref{e75} shows that we may use the perturbative solution of $v_k$
and $v_{k'}$ in order to arrive at an expression for $E_3^{(0)}(k,k')$ in the
regime we are interested in.

Let me now suppose that $E_3^{(0)}(k,k')$ sits in between $E_1(k)$ and
$E_1(k')$ and see if this is ``legal''. For simplicity, assume $-|k| \le k' \le
|k|$ and 
\begin{align}
		E_1(k') \le E_3^{(0)}(k,k') \le E_1(k).
		\label{e76}
\end{align}
The defining equation for $E_3^{(0)}$ simplifies to:
\begin{align}
		\label{e77}
		E_3^{(0)}(k,k')
		&=\Bigl|v_k(\ellthreezerokkp)k+v_{k'}(\ellthreezerokkp)k'\Bigr| \\
		&=v_k^{\trb}(\ellthreezerokkp)|k| \left|1+\FR{v_{0}(\ellthreezerokkp)k'}{v_k^{\trb}(\ellthreezerokkp)k}\right| \\
		%&=v_k^{\trb}(\ellthreezerokkp)|k| \left|1+\FR{k'}{k}\FR{1-2\PFR{\ellthreezerokkp-\ellonek}{\ellonek+\ell_0}}{1-\FR{\ellthreezerokkp-\ellonek}{\ellonek+\ell_0}}\right| \\
		\label{e78}
		&=v_k^{\trb}(\ellthreezerokkp)|k| \left|1+\FR{k'}{k}\left(1-\FR{\ellthreezerokkp-\ellonek}{\ellonek+\ell_0}\right)\right| 
\end{align}
We can solve for $\ellthreezerokkp-\ell_0$ assuming $\ellthreezerokkp-\ell_0 \ll
1$ and $\ellonek+\ell_0\gg1$. 
\begin{align}
		\label{e79}
		\Lambda_fe^{-\ellthreezerokkp}
		&=v_k^{\trb}(\ellthreezerokkp)|k|(1+k'/k) \\
		%\Lambda_fe^{-\ellonek}
		E_1(k)
		\left[1-(\ellthreezerokkp-\ellonek)\right]
		&=v_0(\ellonek)\left[1-\FR{\ellthreezerokkp-\ellonek}{\ellonek+\ell_0}\right]\left|k+k'\right| \\
		(\ellthreezerokkp - \ellonek) &=
		\FR{1-k'/k}{2}
		\left( 1+\FR{1+k'/k}{2(\ellonek+\ell_0)} \right)
\end{align}
Here $1+k'/k \sim \mathcal O(1)$ which means that there exists a perturbative
solution to $\ellthreezerokkp$. The logarithmic width of the intermediate region
is of order $\elltwok-\ellonek=\log(\ellonek+\ell_0) \ge \log\ell_0 \gg 1$, and
so the fact that $\ellthreezerokkp - \ellonek \sim \mathcal O(1)$ means that we
may essentially treat $\ellthreezerokkp = \ellonek$:
\begin{align}
		E_3^{(0)}(k,k') 
		&= E_1(k)\left[
				1 - \FR{1-k'/k}{2} \left( 1+\FR{1+k'/k}{2(\ellonek+\ell_0)} \right)
		\right].
		\label{e82}
\end{align}

In the case if $E_3^{(0)} \le E_1(k') \le E_1(k)$, then \eqref{e79} is still
a good approximation to \eqref{e78} which makes \eqref{e82} still valid. 

Let us summarize the results that we have obtained starting from \eqref{e64}.
The full crossover energy scale, $E_3(k,k')$, is the largest of three crossover
scales $E_3^{(0)}(k,k')$, $E_2(k)$, $E_2(k')$. When it happens that,
$E_3^{(0)}(k,k')\ge E_2(k),E_2(k')$, then for $|k'| < |k|$, $E_3(k,k')$ is given
by \eqref{e82}. When the expression in \eqref{e82} is smaller than $E_2(k)$ or
$E_2(k')$, then $E_3(k,k') = \max(E_2(k),E_2(k'))$.
\begin{align}
		E_3(k,k') &= 
		\max\left(
		\max \left[
		E_1(k), E_1(k')
		\right] 
		\left[ 1 - \FR{1-\sigma_{k,k'}\mf m_{k,k'}/\mf M_{k,k'}}{2} \left(
						1+\FR{1+\sigma_{k,k'}\mf m_{k,k'}/\mf M_{k,k'}}{2(\min(\ellonek,\ellonekp)+\ell_0)}
		\right) \right],
		E_2(k),
		E_2(k')
		\right)
		\\
		  &\approx \max\left(
		\max \left[
		E_1(k), E_1(k')
		\right] 
	    %\left[ \FR{1}{2} + \FR{\sigma_{k,k'}\mf m_{k,k'}}{2\mf M_{k,k'}} \right],
		\left[ \FR{|k+k'|}{2\mf M_{k,k'}} \right],
		E_2(k),
		E_2(k')
		\right),
		\label{e82final}
		\\
		\sigma_{k,k'} &= \sgn(k\cdot k'),\quad
		\mathfrak m_{k,k'} = \min(|k|,|k'|),\quad
		\mathfrak M_{k,k'} = \max(|k|,|k'|).
\end{align}
The expression in \eqref{e82final} is the explicit expression of $E_3(k,k')$ in
terms of $E_1,E_2$ (cf. \eqref{eqn165}, \eqref{eqn170}, \eqref{e207}). Let us
write a simpler expression of \eqref{e82final} in the case when $|k| > |k'|$:
\begin{align}
		E_3(k,k')
				&= \max( E_1(k) \FR{|k+k'|}{2|k|}, E_2(k) )
		\label{e82a}
		\\
				&\approx \max( v_0 |k+k'|, 2v_0c_0|k| )
\end{align}
Yet another way to write \eqref{e82final} is very simply:
\begin{align}
		E_3(k,k') &= \max( E_1\Bigl(\FR{k+k'}2\Bigr), E_2(k), E_2(k') )
		\\
		\ellthreekkp &= \min\Bigl(\ell^{(1)}_{(k+k')/2},\elltwok,\elltwokp\Bigr)
\end{align}

\subsubsection{Flow of Off-Diagonal Yukawa Coupling}

The off-diagonal beta function is given by:
\begin{align}
\widehat\beta^{(g)}_{k,k'} &=
\FR{g_{k,k'}}{z(\ell)}\left( 
\left[
		-\FR{1}{2\pi N_cN_f}w_0(\ell)\log\PFR{1}{w_0(\ell)}
		+\FR{N_c^2-1}{2\pi N_cN_f}w_0(\ell)
		-\FR{N_c^2-1}{\pi^2N_cN_f}v_0(\ell)\log\PFR{1}{c(\ell)}
		-\FR{N_c^2-1}{8\pi^2N_c^2N_f^2}w_0(\ell)^2\log^2\PFR{1}{w_0(\ell)}
\right]
\right.\nonumber\\
&\hspace{1.5cm}\left.
		+\FR{2g_{k,k}(\ell)g_{k',k'}(\ell)}{\pi^2N_cN_fc(\ell)(V_{F,k}(\ell)+V_{F,k'}(\ell))}
		\log\PFR{(V_{F,k}(\ell)^{-1}+V_{F,k}(\ell)^{-1})c}{v_k(\ell)+v_{k'}(\ell)}\Theta(\ell^{(3)}_{kk'}-\ell)
		-\FR{(N_c^2-1)g_{k,k}(\ell)^2    \Theta(\ell^{(2)}_{k }-\ell) }{2\pi^2N_cN_f c(\ell)V_{F,k}(\ell) }
\right.\nonumber\\
&\hspace{1.5cm}\left.
		-\FR{(N_c^2-1)g_{k',k'}(\ell)^2 \Theta(\ell^{(2)}_{k'}-\ell)
		}{2\pi^2N_cN_fc(\ell)V_{F,k'}(\ell)}
		-\FR{(N_c^2-1)}{4\pi^4N_c^2N_f^2}\FR{g_{k ,k }(\ell)^4}{c(\ell)^2V_{F,k
		}(\ell)^2}\log^2\PFR{v_{k }(\ell)}{c(\ell)V_{F,k}(\ell)}\Theta(\ell^{(1)}_{k }-\ell)
\right.\nonumber\\
&\hspace{1.5cm}\left.
	%%%%
		-\FR{(N_c^2-1)}{4\pi^4N_c^2N_f^2}\FR{g_{k',k'}(\ell)^4}{c(\ell)^2V_{F,k'}(\ell)^2}\log^2\PFR{v_{k'}(\ell)}{c(\ell)V_{F,k'}(\ell)}\Theta(\ell^{(1)}_{k'}-\ell)
\right)
\label{betaGgen}
\end{align}

\noindent In the high-energy regime, $\ell \le \ellonek,\ellonekp$ the flow of
$g_{k,k'}$ is the same as at the hot spot:
\begin{align}
g_{k,k'}^{\tra}(\ell) &= \sqrt{\FR{\pi^3 N_c N_f}{4(N_c^2-1)} \FR{1}{(\ell+\ell_0)\log(\ell+\ell_0)}}
\end{align}

\noindent 
In order to study the intermediate regime, let us consider the the case when
$|k| > |k'|$. There are at most two intermediate regimes for the off-diagonal
coupling, $g_{k,k'}$. In the region satisfying $|k+k'| > c|k|$, there are two
regimes, $(\ellthreekkp,\elltwok)$ and $(\elltwok,\elltwokp)$. Whereas in the
regime where $|k+k'| < c|k|$ we have only one intermediate regime $(\elltwok,
\elltwokp)$. 

\begin{list}{}{}{}
\item[({\color{red}$i$})]

		First, let us consider the region $|k+k'| > c|k|$ and explain the
		intermediate behaviour of $g_{k,k'}$. In this region the crossover
		scales satisfy $\ellonek \le \ellthreekkp \le \elltwok \le \elltwokp$.
		Note that I have not included $\ellonekp$ in the above inequalities
		because it is possible that $\ellonekp$ either satisfies $\ellonek \le
		\ellonekp \le \ellthreezerokkp$ or $\ellonek \le \ellthreezerokkp \le
		\ellonekp$. Regardless, we shall soon see that neither $\ellonek$ nor
		$\ellonekp$ affects the qualitative behaviour of the flow of $g_{k,k'}$.

		For $\ellonek \le \ell \le \ellthreekkp$ the beta function,
		\eqref{betaGgen}, for $g_{k,k'}$ takes the form:
		\begin{align}
				&\widehat\beta^{(g)}_{k,k'}(\ellonek \le \ell \le
				\min(\ellthreekkp,\ellonekp))
				\nonumber\\&= 
				\FR{g_{k,k'}(\ell)}{z(\ell)}\left( 
\left[
		-\FR{1}{2\pi N_cN_f}w_0(\ell)\log\PFR{1}{w_0(\ell)}
		+\FR{N_c^2-1}{2\pi N_cN_f}w_0(\ell)
		-\FR{N_c^2-1}{\pi^2N_cN_f}v_0(\ell)\log\PFR{1}{c(\ell)}
		-\FR{N_c^2-1}{8\pi^2N_c^2N_f^2}w_0(\ell)^2\log^2\PFR{1}{w_0(\ell)}
\right]
\right.\nonumber\\
&\hspace{1.5cm}\left.
		+\FR{2g_{k,k}(\ell)g_{k',k'}(\ell)}{\pi^2N_cN_fc(\ell)(V_{F,k}(\ell)+V_{F,k'}(\ell))}
		\log\PFR{(V_{F,k}(\ell)^{-1}+V_{F,k}(\ell)^{-1})c(\ell)}{v_k(\ell)+v_{k'}(\ell)}
						   %\Theta(\ell^{(3)}_{kk'}-\ell)
		-\FR{(N_c^2-1)g_{k,k}(\ell)^2    %\Theta(\ell^{(2)}_{k }-\ell) 
		}{2\pi^2N_fN_fc(\ell)V_{F,k}(\ell) }
\right.\nonumber\\
&\hspace{1.5cm}\left.
		-\FR{(N_c^2-1)g_{k',k'}(\ell)^2  %\Theta(\ell^{(2)}_{k'}-\ell)  
		}{2\pi^2N_cN_fc(\ell)V_{F,k'}(\ell)}
%-\FR{(N_c^2-1)}{4\pi^4N_c^2N_f^2c^2V_{F,k }^2}\FR{g_{k ,k }^4}{c^2V_{F,k }^2}\log^2\PFR{v_{k }}{cV_{F,k}}\Theta(\ell^{(1)}_{k }-\ell)
%\right.\nonumber\\
%&\hspace{1.5cm}\left.
	%%%%
		-\FR{(N_c^2-1)}{4\pi^4N_c^2N_f^2}\FR{g_{k',k'}(\ell)^4}{c(\ell)^2V_{F,k'}(\ell)^2}
		\log^2\PFR{v_{k'}(\ell)}{c(\ell)V_{F,k'}(\ell)}
						   %\Theta(\ell^{(1)}_{k'}-\ell)
\right)
		\end{align}
		This beta function differs from its' high energy counterpart by a term
		of order $w^2\log^2w$. Assuming $\ell_0$ is large, we can solve for the
		flow perturbatively in the parameter $\ell-\ellonek$, just as we did
		when solving for the diagonal flow. The result is:
		\begin{align}
				g_{k,k'}^{\trb_0}(\ell)
				&= 
				g_{k,k'}^{\tra}(\ellonek)
				\left[ 1 - (\ell-\ellonek) \cdot v_0(\ellonek) \log \FR{1}{c(\ellonek)}\FR{7(N_c^2-1)}{4N_cN_f} \right]
				\\
				&\approx
				g_{k,k'}^{\tra}(\ellonek)
				\left[ 1 - \FR{7}{16}\FR{\ell-\ellonek}{\ellonek+\ell_0} \right]
		\end{align}
		%useful relation hot spot
		%using $w^2\log^2w = 4 N_c N_f v \log (1/c)$
		As we saw earlier, this flow is typical of the flow of the hot spot
		flow. As a result we will not treat the scale $\ellonek$ nor
		$\ellonekp$ as a crossover scale because it does changes the flow of the
		off-diagonal $g_{k,k'}$ very weakly (of order $v_0\log(1/c_0)$).

		Let us now consider the first true intermediate regime $(\ellthreekkp,\elltwok)$.
		The beta function in this regime is given by:
		\begin{align}
				&\widehat\beta^{(g)}_{k,k'}(\ellthreekkp \le \ell \le \elltwok)
				\nonumber\\&= 
				\FR{g_{k,k'}(\ell)}{z(\ell)}\left( 
\left[
		-\FR{1}{2\pi N_cN_f}w_0(\ell)\log\PFR{1}{w_0(\ell)}
+\FR{N_c^2-1}{2\pi N_cN_f}w_0(\ell)
-\FR{N_c^2-1}{\pi^2N_cN_f}v_0(\ell)\log\PFR{1}{c(\ell)}
-\FR{N_c^2-1}{8\pi^2N_c^2N_f^2}w_0(\ell)^2\log^2\PFR{1}{w_0(\ell)}
\right]
\right.\nonumber\\
&\hspace{1.5cm}\left.
		%+\FR{2g_{k,k}g_{k',k'}}{\pi^2N_cN_fc(V_{F,k}+V_{F,k'})}\log\PFR{(V_{F,k}^{-1}+V_{F,k}^{-1})c}{v_k+v_{k'}}
						   %\Theta(\ell^{(3)}_{kk'}-\ell)
		-\FR{(N_c^2-1)g_{k,k}(\ell)^2    %\Theta(\ell^{(2)}_{k }-\ell) 
		}{2\pi^2N_cN_fc(\ell)V_{F,k}(\ell) }
%\right.\nonumber\\
%&\hspace{1.5cm}\left.
		-\FR{(N_c^2-1)g_{k',k'}(\ell)^2  %\Theta(\ell^{(2)}_{k'}-\ell)  
		}{2\pi^2N_cN_fc(\ell)V_{F,k'}(\ell)}
%-\FR{(N_c^2-1)}{4\pi^4N_c^2N_f^2c^2V_{F,k }^2}\FR{g_{k ,k }^4}{c^2V_{F,k }^2}\log^2\PFR{v_{k }}{cV_{F,k}}\Theta(\ell^{(1)}_{k }-\ell)
%\right.\nonumber\\
%&\hspace{1.5cm}\left.
	%%%%
		-\FR{(N_c^2-1)}{4\pi^4N_c^2N_f^2}\FR{g_{k',k'}(\ell)^4}{c(\ell)^2V_{F,k'}(\ell)^2}
		\log^2\PFR{v_{k'}(\ell)}{c(\ell)V_{F,k'}(\ell)}
						   %\Theta(\ell^{(1)}_{k'}-\ell)
\right)
		\end{align}
		Solving for the flow perturbatively in $\ell-\ellthreekkp$, we get:
		\begin{align}
				g_{k,k'}^{\trb_1}(\ell)
				&= 
				g_{k,k'}^{\tra}(\ellthreekkp)
				\left[ 1 - (\ell-\ellthreekkp) \cdot \left( \FR{7(N_c^2-1)}{4\pi^2N_cN_f}v_0(\ellthreekkp)\log\FR{1}{c(\ellthreekkp)} + \FR{1}{2\pi N_cN_f}w_0(\ellthreekkp)\log\FR{1}{w_0(\ellthreekkp)}  \right)  \right]
				\\
				&\approx
				g_{k,k'}^{\tra}(\ellthreekkp)
				\left[ 1 
				- \FR{\ell-\ellthreekkp}{2\sqrt{(N_c^2-1)(\ellthreekkp+\ell_0)}} 
				- \FR{7}{16}\FR{\ell-\ellthreekkp}{\ellthreekkp+\ell_0} 
		\right]
		\label{e93}
		\end{align}

		Using the perturbative flow, we may identify the most important
		contributions to the flow of $g_{k,k'}^{\trb_1}$:

		\begin{align}
				\widehat\beta^{(g)}_{k,k'}(\ellthreekkp \le \ell \le \elltwok)
				&\approx
				g_{k,k'}(\ell)\left( 
						-\FR{1}{2\pi N_cN_f}w_0(\ell)\log\PFR{1}{w_0(\ell)}
						-\FR{7(N_c^2-1)}{4\pi^2N_cN_f}v_0(\ell)\log\PFR{1}{c(\ell)}
\right)
\\
				&=
g_{k,k'}^{\trb_1}(\ell)
\left(
		-\FR{1}{2\sqrt{N_c^2-1}}\FR{1}{\sqrt{\ell+\ell_0}}
		-\FR{7}{16}\FR{1}{\ell+\ell_0}
\right)
		\end{align}		

		Integrating:
		\begin{align}
				g_{k,k'}^{\trb_1}(\ellthreekkp \le \ell \le \elltwok)
				&=
				g_{k,k'}^{\tra}(\ellthreekkp)
				\exp\left(
						-\FR{\sqrt{\ell+\ell_0}-\sqrt{\ellthreekkp+\ell_0}}{\sqrt{N_c^2-1}}
						-\FR{7}{16}\log\PFR{\ell+\ell_0}{\ellthreekkp+\ell_0}
				\right)
				\label{eqn100}
		\end{align}

		In the large $\ell_0$ limit, the first term in the argument of the
		exponential in \eqref{eqn100} is larger than the second term and so we
		can simply write:
		\begin{align}
				g_{k,k'}^{\trb_1}(\ellthreekkp \le \ell \le \elltwok)
				&=
				g_{k,k'}^{\tra}(\ellthreekkp)
				\exp\left(
						-\FR{\sqrt{\ell+\ell_0}-\sqrt{\ellthreekkp+\ell_0}}{\sqrt{N_c^2-1}}
				\right)
				\label{eqn101}
		\end{align}

		This is characteristic of the flow of the diagonal Yukawa coupling
		after the high-intermediate energy transition.

		Now, we turn to the second intermediate regime $(\elltwok,\elltwokp)$
		defined by the beta function:
		\begin{align}
				&\widehat\beta^{(g)}_{k,k'}(\elltwok \le \ell \le \elltwokp)
				\nonumber\\&= 
				\FR{g_{k,k'}(\ell)}{z(\ell)}\left( 
\left[
		-\FR{1}{2\pi N_cN_f}w_0(\ell)\log\PFR{1}{w_0(\ell)}
+\FR{N_c^2-1}{2\pi N_cN_f}w_0(\ell)
-\FR{N_c^2-1}{\pi^2N_cN_f}v_0(\ell)\log\PFR{1}{c(\ell)}
-\FR{N_c^2-1}{8\pi^2N_c^2N_f^2}w_0(\ell)^2\log^2\PFR{1}{w_0(\ell)}
\right]
\right.\nonumber\\
&\hspace{1.5cm}\left.
		%+\FR{2g_{k,k}g_{k',k'}}{\pi^2N_cN_fc(V_{F,k}+V_{F,k'})}\log\PFR{(V_{F,k}^{-1}+V_{F,k}^{-1})c}{v_k+v_{k'}}
						   %\Theta(\ell^{(3)}_{kk'}-\ell)
%-\FR{(N_c^2-1)g_{k,k}^2    %\Theta(\ell^{(2)}_{k }-\ell) 
%}{2\pi^2N_fN_fcV_{F,k} }
%\right.\nonumber\\
%&\hspace{1.5cm}\left.
		-\FR{(N_c^2-1)g_{k',k'}(\ell)^2  %\Theta(\ell^{(2)}_{k'}-\ell)  
		}{2\pi^2N_cN_fc(\ell)V_{F,k'}(\ell)}
%-\FR{(N_c^2-1)}{4\pi^4N_c^2N_f^2c^2V_{F,k }^2}\FR{g_{k ,k }^4}{c^2V_{F,k }^2}\log^2\PFR{v_{k }}{cV_{F,k}}\Theta(\ell^{(1)}_{k }-\ell)
%\right.\nonumber\\
%&\hspace{1.5cm}\left.
	%%%%
		-\FR{(N_c^2-1)}{4\pi^4N_c^2N_f^2}\FR{g_{k',k'}(\ell)^4}{c(\ell)^2V_{F,k'}(\ell)^2}\log^2\PFR{v_{k'}(\ell)}{c(\ell)V_{F,k'}(\ell)}
						   \Theta(\ell^{(1)}_{k'}-\ell)
\right)
		\label{e60beta}
		\end{align}
		When writing the above beta function, \eqref{e60beta}, I have explicitly
		added the theta function dependence on $\ellonekp$. As was noted
		previously, it's presence does not change the leading order behaviour
		of the flow of $g_{k,k'}$ but for completeness I have included it.
		The flow of $g_{k,k'}^{\trb_2}$ perturbatively in $\ell-\elltwok$ is given by:
		\begin{align}
				g_{k,k'}^{\trb_2}(\ell)
				&= 
				g_{k,k'}^{\trb_1}(\elltwok)
				\left[ 1 - (\ell-\elltwok) \cdot \left( \FR{7(N_c^2-1)}{4\pi^2N_cN_f}v_0(\elltwok)\log\FR{1}{c(\elltwok)} + \FR{1}{2\pi N_cN_f}w_0(\elltwok)\log\FR{1}{w_0(\elltwok)} - \FR{N_c^2-1}{4\pi N_c N_f}w_0(\elltwok)  \right)  \right]
				\\
				&\approx
				g_{k,k'}^{\trb_1}(\elltwok)
				\left[ 1 
				- \FR{\ell-\elltwok}{\sqrt{(N_c^2-1)(\elltwok+\ell_0)}} 
				- \FR{(\ell-\elltwok)\sqrt{N_c^2-1}}{2\sqrt{(\elltwok+\ell_0)}\log(\elltwok+\ell_0)} 
				- \FR{7}{16}\FR{\ell-\elltwok}{\elltwok+\ell_0} 
		\right]
		\label{e96}
		\end{align}

		Strictly speaking, the regime $(\elltwok,\elltwokp)$ can be very large,
		for example when we are considering $k \ne 0$ and $k'=0$ ($g_{k,0}$).
		If $\elltwokp$ is very large, then a perturbative analysis is not valid. 
		Nonetheless, the perturbative analysis shows which terms in the beta
		function play the dominant role in the flow of $g_{k,k'}$. In the large
		$\elltwokp$ limit, the beta function for $g_{k,k'}$ in the regime
		$(\elltwok,\elltwokp)$ can be approximated as:
		\begin{align}
				\widehat\beta^{(g)}_{k,k'}(\elltwok \le \ell \le \elltwokp)
				&= 
				\FR{g_{k,k'}(\ell)}{z(\ell)}\left( 
\left[
		-\FR{1}{2\pi N_cN_f}w_0(\ell)\log\PFR{1}{w_0(\ell)}
+\FR{N_c^2-1}{2\pi N_cN_f}w_0(\ell)
\right]
-\FR{(N_c^2-1)g_{k',k'}(\ell)^2  %\Theta(\ell^{(2)}_{k'}-\ell)  
}{2\pi^2N_cN_fc(\ell)V_{F,k'}(\ell)}
\right)
		\label{e60betaApprox1}
		\\
				  &= 
				  \FR{g_{k,k'}(\ell)}{z(\ell)}\left( 
						  -\FR{1}{2\pi N_cN_f}w_0(\ell)\log\PFR{1}{w_0(\ell)}
						  +\FR{N_c^2-1}{4\pi N_cN_f}w_0(\ell)
\right)
		\label{e60betaApprox2}
		\end{align}
		To be totally precise, going from \eqref{e60betaApprox1} to
		\eqref{e60betaApprox2} I have assumed that $\ell \le \ellonekp$, but
		as we have seen in earlier sections the flow of $g_{k',k'}$ between
		$\ellonekp$ and $\elltwokp$ is very small and so to a good approximation
		we can assume the hot spot flow for $g_{k',k'}$ all the way to
		$\elltwokp$ to simplify the current analysis.  The flow of $g_{k',k'}$
		following \eqref{e60betaApprox2} is given by:
		\begin{align}
		\begin{split} 
				\label{e99}
				g_{k,k'}^{\trb_2}(\ell)&=
				g_{k,k'}^{\trb_1}(\elltwok)
		\exp\left(
		- \FR{\sqrt{\ell+\ell_0}-\sqrt{\elltwok+\ell_0}}{\sqrt{N_c^2-1}}
		+
		\FR{\sqrt{N_c^2-1}}{2} \left[
		\mathrm{Ei}\left(\FR{1}{2}\log(\ell+\ell_0)\right)-\mathrm{Ei}\left(\FR{1}{2}\log(\elltwok+\ell_0)\right)
		\right]
		\right)
		\end{split}
		\end{align}

		Beyond $\elltwokp$ the beta function is equivalent to that of the
		low-energy diagonal Yukawa coupling:
		\begin{align}
				\widehat\beta^{(g)}_{k,k'}(\elltwok \le \ell \le \elltwokp)
				  &= 
				  \FR{g_{k,k'}(\ell)}{z(\ell)}\left( 
						  -\FR{1}{2\pi N_cN_f}w_0(\ell)\log\PFR{1}{w_0(\ell)}
						+\FR{N_c^2-1}{2\pi N_cN_f}w_0(\ell)
						\right)
		\end{align}
		whose asymptotic solution is:
		\begin{align}
		\begin{split}
				\label{e101}
				g_{k,k'}^{\trc}(\ell)&=
				g_{k,k'}^{\trb_2}(\elltwokp)
		\exp\left(
		- \FR{\sqrt{\ell+\ell_0}-\sqrt{\elltwokp+\ell_0}}{\sqrt{N_c^2-1}}
		+
		\sqrt{N_c^2-1}\left[
		\mathrm{Ei}\left(\FR{1}{2}\log(\ell+\ell_0)\right)-\mathrm{Ei}\left(\FR{1}{2}\log(\elltwokp+\ell_0)\right)
		\right]
		\right)
		\end{split}
		\end{align}

		In summary:
		\begin{align}
				\hspace{-1.5cm}
				g_{k,k'}(\ell)
				&=
				\begin{cases}
			%\left\{
			%\begin{aligned}
				g_{k,k'}^{\tra}(\ell)\equiv
						\sqrt{\FR{\pi^3 N_c N_f}{4(N_c^2-1)}\FR{1}{(\ell+\ell_0)\log(\ell+\ell_0)}}
				& \ell \le \ellthreekkp\\
				g_{k,k'}^{\trb_1}(\ell)\equiv
				g_{k,k'}^{\tra}(\ellthreekkp)
				\exp\left(
						-\FR{\sqrt{\ell+\ell_0}-\sqrt{\ellthreekkp+\ell_0}}{\sqrt{N_c^2-1}}
				\right)
				%
				%
				%	g_{k,k'}^{\tra}(\ellthreekkp)
				%	\left[ 1 
				%	- \FR{\ell-\ellthreekkp}{\sqrt{(N_c^2-1)(\ellthreekkp+\ell_0)}} 
				%	- \FR{7}{16}\FR{\ell-\ellthreekkp}{\ellthreekkp+\ell_0} 
				%	\right]
				& \ellthreekkp \le \ell \le \elltwok\\
				g_{k,k'}^{\trb_2}(\ell)\equiv
						g_{k,k'}^{\trb_1}(\elltwok)
						\exp\left(
						- \FR{\sqrt{\ell+\ell_0}-\sqrt{\elltwok+\ell_0}}{\sqrt{N_c^2-1}}
						+
						\FR{\sqrt{N_c^2-1}}{2}\left[
						\mathrm{Ei}\left(\FR{1}{2}\log(\ell+\ell_0)\right)-\mathrm{Ei}\left(\FR{1}{2}\log(\elltwok+\ell_0)\right)
						\right]
						\right) 
				& \elltwok \le \ell \le \elltwokp\\
				g_{k,k'}^{\trc}(\ell)\equiv
						g_{k,k'}^{\trb_2}(\elltwokp)
						\exp\left(
						- \FR{\sqrt{\ell+\ell_0}-\sqrt{\elltwokp+\ell_0}}{\sqrt{N_c^2-1}}
						+
						\sqrt{N_c^2-1}\left[
						\mathrm{Ei}\left(\FR{1}{2}\log(\ell+\ell_0)\right)-\mathrm{Ei}\left(\FR{1}{2}\log(\elltwokp+\ell_0)\right)
						\right]
						\right) 
				& \ell \ge \elltwokp
				%\end{aligned}
				%\right.
			\end{cases}
		\end{align}

\item[({\color{red}$ii$})]

		Now, let us briefly consider the region $|k+k'| < c|k|$ and explain the
		intermediate behaviour of $g_{k,k'}$. In this region the crossover $k'
		\approx -k$ and so $\elltwok \approx \elltwokp$; moreover, in this
		regime $\ellthreekkp$ is also given by $\elltwok$. Therefore the
		analysis of the previous section holds but with some simplifications.
		The simplification consists of a vanishing of the intermediate regions
		$\trb_1,\trb_2$; since $\ellthreekkp \approx \elltwok \approx
		\elltwokp$. As a result the off-diagonal Yukawa coupling immediately
		enters the low-energy regime at the scale $\ellthreekkp$:
		\begin{align}
				\hspace{-1.5cm}
				g_{k,k'}(\ell)
				&=
				\begin{cases}
			%\left\{
			%\begin{aligned}
				g_{k,k'}^{\tra}(\ell)\equiv
						\sqrt{\FR{\pi^3 N_c N_f}{4(N_c^2-1)}\FR{1}{(\ell+\ell_0)\log(\ell+\ell_0)}}
				& \ell \le \ellthreekkp\\
				g_{k,k'}^{\trc}(\ell)\equiv
						g_{k,k'}^{\tra}(\ellthreekkp)
						\exp\left(
						- \FR{\sqrt{\ell+\ell_0}-\sqrt{\ellthreekkp+\ell_0}}{\sqrt{N_c^2-1}}
						+
						\sqrt{N_c^2-1}\left[
						\mathrm{Ei}\left(\FR{1}{2}\log(\ell+\ell_0)\right)-\mathrm{Ei}\left(\FR{1}{2}\log(\ellthreekkp+\ell_0)\right)
						\right]
						\right) 
				& \ell \ge \ellthreekkp
				%\end{aligned}
				%\right.
			\end{cases}
		\end{align}
\end{list}

\subsubsection{Momentum Dependence of Off-diagonal Yukawa Coupling}

%\begin{figure}[h!]
%		\centering
%		\includegraphics[scale=.4]{./Figures/OffDiagMomentumProfile0.pdf}
%		\includegraphics[scale=.4]{./Figures/OffDiagMomentumProfile1.pdf}
%		\includegraphics[scale=.4]{./Figures/OffDiagMomentumProfile2.pdf}
%		\caption{
%		\label{fig3}
%		Relevant regions for $g(k,k';\mu)$. 
%		}
%\end{figure}
%\textit{Explanation of figure~\ref{fig3}.}
%		Axes: $(x,y) \equiv (k,k')$;
%		Orange: $|k-k'|<\Lambda_b$; %$v_0(k+k') > v_0 c |k| \iff \ellthreekkp < \elltwok,\elltwokp$
%		Blue:   $v_0(k+k') < v_0 c |k| \iff \ellthreekkp = \elltwok = \elltwokp$;
%		Green:  $E_3(k,k') = \max(v_0c|k|,v_0|k+k'|) \le \mu$ (hot spot behaviour).

		The formula for the off-diagonal Yukawa couling that was quoted before
		implicitly assumes that $|k'| < |k|$ and is given by:

		\begin{align}
				\hspace{-1.5cm}
				g_{k,k'}(\ell)
				&=
				\begin{cases}
			%\left\{
			%\begin{aligned}
				g_{k,k'}^{\tra}(\ell)\equiv
						\sqrt{\FR{\pi^3 N_c N_f}{4(N_c^2-1)}\FR{1}{(\ell+\ell_0)\log(\ell+\ell_0)}}
				& \ell \le \ellthreekkp\\
				g_{k,k'}^{\trb_1}(\ell)\equiv
				g_{k,k'}^{\tra}(\ellthreekkp)
				\exp\left(
						-\FR{\sqrt{\ell+\ell_0}-\sqrt{\ellthreekkp+\ell_0}}{\sqrt{N_c^2-1}}
				\right)
				%
				%
				%	g_{k,k'}^{\tra}(\ellthreekkp)
				%	\left[ 1 
				%	- \FR{\ell-\ellthreekkp}{\sqrt{(N_c^2-1)(\ellthreekkp+\ell_0)}} 
				%	- \FR{7}{16}\FR{\ell-\ellthreekkp}{\ellthreekkp+\ell_0} 
				%	\right]
				& \ellthreekkp \le \ell \le \elltwok\\
				g_{k,k'}^{\trb_2}(\ell)\equiv
						g_{k,k'}^{\trb_1}(\elltwok)
						\exp\left(
						- \FR{\sqrt{\ell+\ell_0}-\sqrt{\elltwok+\ell_0}}{\sqrt{N_c^2-1}}
						+
						\FR{\sqrt{N_c^2-1}}{2}\left[
						\mathrm{Ei}\left(\FR{1}{2}\log(\ell+\ell_0)\right)-\mathrm{Ei}\left(\FR{1}{2}\log(\elltwok+\ell_0)\right)
						\right]
						\right) 
				& \elltwok \le \ell \le \elltwokp\\
				g_{k,k'}^{\trc}(\ell)\equiv
						g_{k,k'}^{\trb_2}(\elltwokp)
						\exp\left(
						- \FR{\sqrt{\ell+\ell_0}-\sqrt{\elltwokp+\ell_0}}{\sqrt{N_c^2-1}}
						+
						\sqrt{N_c^2-1}\left[
						\mathrm{Ei}\left(\FR{1}{2}\log(\ell+\ell_0)\right)-\mathrm{Ei}\left(\FR{1}{2}\log(\elltwokp+\ell_0)\right)
						\right]
						\right) 
				& \ell \ge \elltwokp
				%\end{aligned}
				%\right.
			\end{cases}
		\end{align}

		\noindent\emph{Approximate Solution to Off-Diagonal Yukawa Coupling.}

		I think it would be best to simplify the analytics and consider the
		large $\ell_0$ limit. In this case the exponential integral function can
		be ignored compared to the $\sqrt{\ell}$ dependence and so the
		functional dependence of $g(k,k';\mu)$ becomes:
		\begin{align}
				g_{k,k'}(\ell)
				&=
				\begin{cases}
				g_{k,k'}^{\tra}(\ell)\equiv
						\sqrt{\FR{\pi^3 N_c N_f}{4(N_c^2-1)}\FR{1}{(\ell+\ell_0)\log(\ell+\ell_0)}}
				& \ell \le \ellthreekkp\\
				g_{k,k'}^{\trb_1}(\ell)\equiv
				g_{k,k'}^{\tra}(\ellthreekkp)
				\exp\left(
						-\FR{\sqrt{\ell+\ell_0}-\sqrt{\ellthreekkp+\ell_0}}{\sqrt{N_c^2-1}}
				\right)
				& \ell \ge \ellthreekkp
			\end{cases}
		\end{align}

		\noindent
		Another way to write the above equation is:
		\begin{align}
				g_{k,k'}(\ell_\mu)
				&=
\sqrt{\FR{{\pi^3 N_c N_f}/{4(N_c^2-1)}}{(\min(\ell_\mu,\ellthreekkp)+\ell_0)\log(\min(\ell_\mu,\ellthreekkp)+\ell_0)}}
				\exp\left(
		(\sqrt{\ellthreekkp+\ell_0}-\sqrt{\ell+\ell_0})\FR{\theta(\ell_\mu-\ellthreekkp)}{\sqrt{N_c^2-1}}
				\right)
				\label{e114}
		\end{align}

		\noindent In the regime in which $\ell_\mu \ll \ell_0$ we may simplify
		the above expression by expanding and keeping the leading order
		contribution controlled by $1/\ell_0$. Let us use the notation that
		$v \equiv v_0(0)$ and $c = c(0)$:
		
		\begin{align}
				g_{k,k'}(\ell_\mu)
				&=
				\sqrt{\FR{\pi v}{2}}
				\exp\left(
						\FR{\theta(\ell_\mu-\ellthreekkp)}{2\sqrt{\ell_0(N_c^2-1)}}
						\log\PFR{\mu}{E_3(k,k')}
				\right)
				=
				\sqrt{\FR{\pi v}{2}}
				\PFR{\mu}{\max(\mu,E_3(k,k'))}^{(2c/\pi)}
		\end{align}
		where 
		\begin{align}
				E_3(k,k') = \min(\Lambda_f,
				\max(E_1((k+k')/2),E_2(k),E_2(k')))
		\end{align}
		For example, in the case we are in the regime that $k+k' \ll \Lambda_f$, $(k-k')/k \gg c$,
		and $\mu \gg \Lambda_f e^{-\ell_0}$:
		\begin{align}
				g(k,k',\mu) = 
				\sqrt{\FR{\pi v}{2}}
				\PFR{\mu}{v|k+k'|}^{(2c/\pi)}
				\label{solnGKKP}
		\end{align}

%	\begin{figure}[h!]
%			\centering
%			\includegraphics[scale=.6]{./Figures/gkkp1.pdf}
%			\caption{
%			\label{figGKKP1}
%			$\ell_0 = 4$, $\ell = 0.69$, $\Lambda_f=1$.
%			}
%	\end{figure}
%
%	\begin{figure}[h!]
%			\centering
%			\includegraphics[scale=.6]{./Figures/justifyGKKP5.pdf}
%			\caption{
%			\label{figGKKP3}
%			Log-Log Plot of $ c^{(2c/\pi)} $ as a function of $\ell_0$ where
%			$c = \FR{\pi}{4\sqrt{N_c^2-1}}\FR{1}{\sqrt{\ell_0}}$.
%			}
%	\end{figure}

Let's compute the slope of equation \ref{solnGKKP}:
\begin{align}
		\log(g_{k,k',\mu})& \sim - \FR{2c}{\pi} \log k + \text{indep of $k$}\\
\FR{\di \log(g_{k,k',\mu})}{\di k}&\sim - \FR{c}{k}
\end{align}

At $k=\mu/v$, $\Lambda \sim \left|\FR{\di \log(g_{k,k',\mu})}{\di k}\right|^{-1} = \FR{\mu}{v c}$.

\begin{figure}[ht]
		\centering
		\begin{subfigure}[t]{0.45\textwidth}
		\includegraphics[scale=.6]{./gkkp1.pdf}
		\caption{
		\label{figGKKP1}
		$\ell_0 = 4$, $\ell = 0.69$, $\Lambda_f=1$.
		}
		\end{subfigure}
		\begin{subfigure}[t]{0.45\textwidth}
		\includegraphics[scale=.6]{./justifyGKKP5.pdf}
		\caption{
		\label{figGKKP3}
		Log-Log Plot of $ c^{(2c/\pi)} $ as a function of $\ell_0$ where
		$c = \FR{\pi}{4\sqrt{N_c^2-1}}\FR{1}{\sqrt{\ell_0}}$.
		}
		\end{subfigure}
\end{figure}
