# Supplementary material for: Field-theoretic functional renormalization group formalism for non-Fermi liquids and its application to the antiferromagnetic quantum critical metal in two dimensions
Source: arXiv:2208.00730 source file (2023-01-06)
Supplement: Supplementary file 3 [file appendixSYM.tex]

\section{Transformation of the coupling functions under the $C_4$ symmetry}
 \label{appendix:sym}

The Hermiticity of the Hamiltonian and the Grasmann character of the fermionic fields
impose further constraints on the form of the  coupling functions as
\begin{align}
\begin{split}\label{eq:Prps}
%%&\hspace{4.1cm} 
g(x',x) & =  g(x,x')^{*}\\
\lambda^{j_1j_2j_3j_4}_{N_1N_2N_3N_4;\sigma_1\sigma_2\sigma_3\sigma_4}(x_{1},x_{2},x_{3},x_{4})
& =\lambda^{j_4j_3j_2j_1}_{N_4N_3N_2N_1;\sigma_4\sigma_3\sigma_2\sigma_1}(x_{4},x_{3},x_{2},x_{1})^{*}\\
&=-\lambda^{j_2j_1j_3j_4}_{N_2N_1N_3N_4;\sigma_2\sigma_1\sigma_3\sigma_4}(x_{2},x_{1},x_{3},x_{4}) \\
%%\\&\hspace{3.8cm}
& =-\lambda^{j_1j_2j_4j_3}_{N_1N_2N_4N_3;\sigma_1\sigma_2\sigma_4\sigma_3}(x_{1},x_{2},x_{4},x_{3}).
\end{split}
\end{align}
%The momentum-dependent four-fermion coupling functions in the forward scattering channel encode the Landau parameters as a function of the momentum along the FS. These also include non-forward scatterings which can lead to instabilities in the particle-hole and particle-particle channels. 
%
Henceforth, we will refer to 
%the momentum-dependent parameters of the theory 
$\{ v(x) $, $ g(x',x)$, $ V_{\mathrm{F}}(x)$, $\lambda^{\{j_i\}}_{\{N_i\};\{\sigma_i\}}(\{x_{i}\}) \}$ 
as coupling functions collectively. 
The the coupling functions should transform covariantly under the action of the $C_4$ group. 
Let $J^{\{j_i\};n}_{\{N_i\};\{\sigma_i\}}(\{x_{i}\})$ denote any of the coupling functions 
associated with $n$ fermions with $n=2$ or $4$.
%where $i=1,\dots n$. 
Under $C_4$-rotations and $C_4$-reflections, 
the coupling functions transform as
%%First, assuming that the action in Eq. (\ref{eq:Action2}) inherits the microscopic $C_4$-symmetry of the FS requires the momentum dependent parameters in Eq. (\ref{eq:Parameters})  to be $C_4$-covariant. That is, under the action of an element $\mathcal{R}\in C_4$, the slope transforms as
\begin{align}\label{eq:SymmetryProperties}
J^{\{j_i\};n}_{\{N_i\};\{\sigma_i\}}(\{k_{i,N_i}\})
\rightarrow
\sum^{8}_{\{N^{'}_j\}=1} {\bf R}_{N_1N^{'}_1}\cdots {\bf R}_{N_nN'_n} ~   J^{\{j_i\};n}_{\{N^{'}_j\};\{\sigma_i\}}(\{k_{i;N^{'}_j}\}) ,
\end{align}
\noindent where 
%$\mathcal{R}\in C_4$ and
${\bf R}$ is the $8$-dimensional 
representation of the $C_4$ group
defined in the space of hot spot indices.
For example, for
the $\pi/2$ rotation we have
${\bf R}^{\pi/2}_{NN'} =\delta_{N',[N+2]_8}$ 
where $1\leq [x]_{8} \leq 8$ gives the reminder on division of $x$ by 8. 
The action in Eq. (\ref{eq:LukewarmAction}) is also invariant under the  particle-hole transformation,
\begin{align}
\begin{split}\label{eq:PH}
\psi_{N,\sigma,j}(k)&\longrightarrow \mathcal{U}_{\sigma\sigma'}\psi^{\dagger}_{N,\sigma',j}(-k),\\
%\psi^{\dagger}_{N,\sigma,j}(k)&\longrightarrow \psi_{N,\sigma',j}(-k)[\mathcal{U}^\dagger]_{\sigma'\sigma},\\
\Phi(q)&\longrightarrow -\mathcal{U} \Phi(q)^{\mathrm{T}} \mathcal{U}^{\dagger}
%\quad \mathcal{U}\in\mathrm{SU}(N_c),
\end{split}
\end{align}
for $ \mathcal{U} \in SU(N_c)$,
provided that the coupling functions satisfy the conditions 
$v(-x) = v(x)$, 
$V_{\mathrm{F}}(-x) = V_{\mathrm{F}}(x)$,
$g(-{x}',-x) = g^*({x}',{x})$\footnote{
	The theory with $N_c=2$ is a special case 
	where we can choose $\mathcal{U} = i \sigma^y$
	such that $\Phi(q)$ is invariant under the particle-hole transformation.
	This special property is rooted in the fact that the fundamental and anti-fundamental
	representations of SU(2) are the same.
	Whether the field for the collective mode is invariant or not under the particle-hole symmetry in Eq. (\ref{eq:PH}) is not important for us.} and
\begin{align}
\begin{split}
&\hspace{-0.5cm}\lambda^{j_1j_2j_3j_4}_{N_1N_2N_3N_4;\sigma_1\sigma_2\sigma_3\sigma_4}(x_{1},x_{2},x_{3},x_{4})=\\
&\hspace{-0.5cm}\sum^{N_c}_{\{\sigma'_i=1\}}\left[\mathcal{U}^\dagger\right]_{\sigma_4\sigma'_1}\left[\mathcal{U}^{\dagger}\right]_{\sigma_3\sigma'_2}\lambda^{j_4j_3j_2j_1}_{N_4N_3N_2N_1;\sigma'_1\sigma'_2\sigma'_3\sigma'_4}(-x_{4},-x_{3},-x_{2},-x_{1})\mathcal{U}_{\sigma'_3\sigma_2}\mathcal{U}_{\sigma'_4\sigma_1}.
\end{split}
\end{align}
In the presence of the exact particle-hole symmetry,
the position of the hot spots on the FS are protected from quantum corrections.
For general momentum-dependent coupling functions,
the particle-hole symmetry is not an exact symmetry,
and the location of the hot spots can be renormalized
from the ones determined by the bare electronic dispersion. 
In what follows we assume that the action in Eq. (\ref{eq:LukewarmAction}) 
has the exact particle-hole symmetry. 
We further assume that the theory preserves the SU($N_c$)$\times$ SU($N_f$) global symmetry by requiring that the four-fermion couplings are covariant under these transformations:
\begin{align}
\begin{split}
&\lambda^{j_1j_2j_3j_4}_{N_1N_2N_3N_4;\sigma_1\sigma_2\sigma_3\sigma_4}(x_{1},x_{2},x_{3},x_{4}) =\\
&\sum^{N_c}_{\{\sigma'_i=1\}}\left[\mathcal{U}^\dagger\right]_{\sigma_1\sigma'_1}\left[\mathcal{U}^\dagger\right]_{\sigma_2\sigma'_2} \lambda^{j_1j_2j_3j_4}_{N_1N_2N_3N_4;\sigma'_1\sigma'_2\sigma'_3\sigma'_4}(x_{1},x_{2},x_{3},x_{4})\mathcal{U}_{\sigma'_3\sigma_3}\mathcal{U}_{\sigma'_4\sigma_4},
\end{split}\\
\begin{split}
&\lambda^{j_1j_2j_3j_4}_{N_1N_2N_3N_4;\sigma_1\sigma_2\sigma_3\sigma_4}(x_{1},x_{2},x_{3},x_{4}) =\\
&\sum^{N_c}_{\{j'_i=1\}}\left[\mathcal{V}^\dagger\right]_{j_1j'_1}\left[\mathcal{V}^\dagger\right]_{\sigma_2\sigma'_2} \lambda^{j'_1j'_2j'_3j'_4}_{N_1N_2N_3N_4;\sigma_1\sigma_2\sigma_3\sigma_4}(x_{1},x_{2},x_{3},x_{4})\mathcal{V}_{j'_3j_3}\mathcal{V}_{j'_4j_4},
\end{split}
\end{align}
\noindent for $\mathcal{U}\in\mathrm{SU}(N_c)$ and $\mathcal{V}\in\mathrm{SU}(N_f)$. 
The four-fermion coupling functions can be decomposed into the spin symmetric($\s{S}$) and spin antisymmetric ($\s{A}$) channels \cite{CHITOV1,CHITOV2,SENECHAL}:
\begin{align}\label{eq:ST}
\lambda^{\{j_i\}}_{\{N_i\};\{\sigma_i\}}(\{x_{i}\}) = \s{A}^{\sigma_1\sigma_2}_{\sigma_3\sigma_4}\lambda^{\{j_i\};\s{S}}_{\{N_i\}}(\{x_{i}\}) + \s{S}^{\sigma_1\sigma_2}_{\sigma_3\sigma_4}\lambda^{\{j_i\};\s{A}}_{\{N_i\}}(\{x_{i}\}),
\end{align}
\noindent where $\s{A}$ and $\s{S}$ are defined as
\begin{align}
\s{A}^{\sigma_1\sigma_2}_{\sigma_3\sigma_4}&= \delta_{\sigma_1\sigma_4}\delta_{\sigma_2\sigma_3}-\delta_{\sigma_1\sigma_3}\delta_{\sigma_2\sigma_4},\label{eq:Anti}\\
\s{S}^{\sigma_1\sigma_2}_{\sigma_3\sigma_4}&= \delta_{\sigma_1\sigma_4}\delta_{\sigma_2\sigma_3}+\delta_{\sigma_1\sigma_3}\delta_{\sigma_2\sigma_4},\label{eq:Simi}
\end{align}
\noindent and which satisfy the symmetry properties $\s{A}^{\sigma_1\sigma_2}_{\sigma_3\sigma_4}=-\s{A}^{\sigma_2\sigma_1}_{\sigma_3\sigma_4} = -\s{A}^{\sigma_1\sigma_2}_{\sigma_4\sigma_3}$ and $\s{S}^{\sigma_1\sigma_2}_{\sigma_3\sigma_4}=\s{S}^{\sigma_2\sigma_1}_{\sigma_3\sigma_4} = \s{S}^{\sigma_1\sigma_2}_{\sigma_4\sigma_3}$. For $N_c=2$, the symmetric (anti-symmetric) channel corresponds to the spin triplet (singlet) channel. Furthermore, from Eq (\ref{eq:Prps}), it follows that $ \lambda^{\{j_i\};\s{A}}_{\{N_i\}}(\{k_{i}\}) $ $\left[\lambda^{\{j_i\};\s{S}}_{\{N_i\}}(\{k_{i}\}) \right]$ is a fully antisymmetric (symmetric) function with respect to the simultaneous exchange of the first two or last two hot spot, flavor and momentum indices.
