# Supplementary material for: Field-theoretic functional renormalization group formalism for non-Fermi liquids and its application to the antiferromagnetic quantum critical metal in two dimensions
Source: arXiv:2208.00730 source file (2023-01-06)
Supplement: Supplementary file 4 [file appendix_feed.tex]

%%%%%%%%%%%%%%%%%%%%%%%%%%%%%%%%%%
%%%%%%%%%%%%%%%%%%%%%%%%%%%%%%%%%%
%%%%%% 4- fermion quantum correction %%%%%%%%%%%%
%%%%%%%%%%%%%%%%%%%%%%%%%%%%%%%%%%
%%%%%%%%%%%%%%%%%%%%%%%%%%%%%%%%%%

\subsection{Two loop Fermion self energy}

The two loop contributions to the fermion self-energy is given as,

\begin{align}
{\bf \Sigma}^{' \mathrm{2L(a)}}_{N}({\bf k}) 
		=
\frac{1}{4 \mu^2}
\int\dd {\bf q} \int \dd {\bf p} ~ 
N_f \lambda^{\spmqty{M_1 & M_3 \\  N &  M_2};\spmqty{\alpha_1 & \alpha_3 \\ \sigma & \alpha_2}}_{\spmqty{k+q  & p-q \\ k & p }}
\lambda^{\spmqty{N & M_2 \\  M_1 &  M_3};\spmqty{\sigma & \alpha_2 \\ \alpha_1 & \alpha_3}}_{\spmqty{k  & p \\ k+q & p-q }}
	G_{M_1}({\bf k}+{\bf q})
	G_{M_2}({\bf p})
	G_{M_3}({\bf p}-{\bf q}) 
	\label{eq:2LoopFSEprime_a}
\end{align}

\begin{align}
{\bf \Sigma}^{' \mathrm{2L(b)}}_{N}({\bf k}) 
		=
-\frac{1}{4 \mu^2}
\int\dd {\bf q} \int \dd {\bf p} ~
\lambda^{\spmqty{M_1 & M_3 \\  N &  M_2};\spmqty{\alpha_1 & \alpha_3 \\ \sigma & \alpha_2}}_{\spmqty{k+q  & k+p \\ k & k+q+p }}
\lambda^{\spmqty{M_2 & N \\  M_1 &  M_3};\spmqty{\alpha_2 & \sigma \\ \alpha_1 & \alpha_3}}_{\spmqty{k+q+p  & k \\ k+q & k+p }}
	G_{M_1}({\bf k}+{\bf q})
	G_{M_2}({\bf k}+{\bf q}+{\bf p})
	G_{M_3}({\bf k}+{\bf p})
	\label{eq:2LoopFSEprime_b}
\end{align}

\begin{align}	
{\bf \Sigma}^{' \mathrm{2L(c)}}_{N}({\bf k}) 
		=
-\frac{1}{4 \mu^2}
\int\dd {\bf q} \int \dd {\bf p}~ \lambda^{\spmqty{M_1 & N \\  N &  M_3};\spmqty{\alpha_1 & \sigma \\ \sigma & \alpha_3}}_{\spmqty{k+q  & k \\ k & k+q }}
\lambda^{\spmqty{M_2 & M_3 \\  M_1 &  M_2};\spmqty{\alpha_2 & \alpha_3 \\ \alpha_1 & \alpha_2}}_{\spmqty{k+q+p  & k+q \\ k+q & k+p+q }}
	G_{M_1}({\bf k}+{\bf q})
	G_{M_2}({\bf k}+{\bf q}+{\bf p})
	G_{M_3}({\bf k}+{\bf q}) 	
	\label{eq:2LoopFSEprime_c}
\end{align}

\subsubsection{Involving hot spots $1$ and $5$ only}

In this section, we consider cases which involves nested channels. For $(N,M_1,M_2,M_3) = (1,1,5,5)$, we have from Eq.~\eqref{eq:2LoopFSEprime_a},

\begin{align}
{\bf \Sigma}^{' \mathrm{2L(a)}}_{1}({\bf k}) 
		=
\frac{N_f}{4 \mu^2}
\int\dd {\bf q} \int \dd {\bf p} ~ 
 \lambda^{\spmqty{1 & 5 \\  1 &  5};\spmqty{\alpha_1 & \alpha_3 \\ \sigma & \alpha_2}}_{\spmqty{k+q  & p-q \\ k & p }}
\lambda^{\spmqty{1 & 5 \\  1 &  5};\spmqty{\sigma & \alpha_2 \\ \alpha_1 & \alpha_3}}_{\spmqty{k  & p \\ k+q & p-q }}
	G_{1}({\bf k}+{\bf q})
	G_{5}({\bf p})
	G_{5}({\bf p}-{\bf q}) ~,
\end{align}

with the explicit form of the fermion propagators, we have, 

\begin{align}\nonumber
{\bf \Sigma}^{' \mathrm{2L(a)}}_{1}({\bf k}) 
		=
\frac{N_f}{4 \mu^2}
\int \frac{\dd {\bf q}\dd {\bf p}}{V_{F, k+q}V_{F, p}V_{F, p-q}}  
 \lambda^{\spmqty{1 & 5 \\  1 &  5};\spmqty{\alpha_1 & \alpha_3 \\ \sigma & \alpha_2}}_{\spmqty{k+q  & p-q \\ k & p }}
\lambda^{\spmqty{1 & 5 \\  1 &  5};\spmqty{\sigma & \alpha_2 \\ \alpha_1 & \alpha_3}}_{\spmqty{k  & p \\ k+q & p-q }}
	\frac{1}{i(k_0+q_0)/V_{F, k+q}+v_{k+q}(k_x+q_x)+k_y+q_y}\times\\
	\frac{1}{ip_0/V_{F, p}-v_{p}p_x-p_y}~
	\frac{1}{i(p_0-q_0)/V_{F, p-q} -v_{p-q}(p_x-q_x)-p_y+q_y}~.
\end{align}

Integrating $p_y$ first, we get,

\begin{align}\nonumber
{\bf \Sigma}^{' \mathrm{2L(a)}}_{1}({\bf k}) 
		=
\frac{N_f}{4 \mu^2}
\int \frac{\dd {\bf q}\dd p_x \dd p_0}{8\pi^3V_{F, k+q}V_{F, p}V_{F, p-q}}  
 \lambda^{\spmqty{1 & 5 \\  1 &  5};\spmqty{\alpha_1 & \alpha_3 \\ \sigma & \alpha_2}}_{\spmqty{k+q  & p-q \\ k & p }}
\lambda^{\spmqty{1 & 5 \\  1 &  5};\spmqty{\sigma & \alpha_2 \\ \alpha_1 & \alpha_3}}_{\spmqty{k  & p \\ k+q & p-q }}
\frac{1}{i(k_0+q_0)V^{-1}_{F, k+q}+v_{k+q}(k_x+q_x)+k_y+q_y}\times\\
	\frac{i\pi\left[{\rm sgn}(p_0-q_0) - {\rm sgn}(p_0)\right]}{ip_0\left(V^{-1}_{F,p-q} - V^{-1}_{F,p}\right) - v_{p-q}(p_x-q_x) + q_y
	+ v_pp_x - iq_0 V^{-1}_{F,p-q}}~.
\end{align}

Now, integrating $q_y$ and simplifying the resulting expression, we obtain,
\begin{align}\nonumber
{\bf \Sigma}^{' \mathrm{2L(a)}}_{1}({\bf k}) 
		=
\frac{N_f}{4 \mu^2}
\int \frac{\dd q_x \dd q_0\dd p_x \dd p_0}{64\pi^4V_{F, k+q}V_{F, p}V_{F, p-q}}  
 \lambda^{\spmqty{1 & 5 \\  1 &  5};\spmqty{\alpha_1 & \alpha_3 \\ \sigma & \alpha_2}}_{\spmqty{k+q  & p-q \\ k & p }}
\lambda^{\spmqty{1 & 5 \\  1 &  5};\spmqty{\sigma & \alpha_2 \\ \alpha_1 & \alpha_3}}_{\spmqty{k  & p \\ k+q & p-q }}
\times\\
	\frac{\left[{\rm sgn}(p_0-q_0) - {\rm sgn}(p_0)\right]\left[{\rm sgn}(k_0+q_0) - {\rm sgn}\left(p_0-p_0V_{F,p-q}V^{-1}_{F,p} - q_0\right)\right]}{ip_0\left(V^{-1}_{F,p-q} - V^{-1}_{F,p}\right) - iq_0\left(V^{-1}_{F,k+q} + V^{-1}_{F,p-q}\right) - ik_0 V^{-1}_{F,k+q} - \Delta_{k,p,q}}~,
\end{align}
where, 
\begin{align}
\Delta_{k,p,q} = (v_{p-q}-v_p)p_x - (v_{p-q}-v_{k+q})q_x + (v_{k+q}-v_k)k_x + \varepsilon_1({\vec k},v_k)~.
\end{align}
\noindent Next, doing the $p_0 ~(|p_0| < \Lambda)$ integration followed by $q_0 ~(|q_0| < \Lambda)$ integration and keeping the dominant contribution, we get,

\begin{align}\nonumber
{\bf \Sigma}^{' \mathrm{2L(a)}}_{1}({\bf k}) 
		=
\frac{N_f }{64 \pi^4\mu^2}\int \frac{\dd q_x\dd p_x}{(V_{F, k+q}+V_{F, p})(V_{F, k+q}+V_{F, p-q})}  
 \lambda^{\spmqty{1 & 5 \\  1 &  5};\spmqty{\alpha_1 & \alpha_3 \\ \sigma & \alpha_2}}_{\spmqty{k+q  & p-q \\ k & p }}
\lambda^{\spmqty{1 & 5 \\  1 &  5};\spmqty{\sigma & \alpha_2 \\ \alpha_1 & \alpha_3}}_{\spmqty{k  & p \\ k+q & p-q }}\times\\
	(ik_0+V_{F,k+q}\Delta_{k,p,q})\log\left[\frac{\Lambda}{\sqrt{k_0^2 + V^2_{F,k+q}\Delta^2_{k,p,q}}\sqrt{k_0^2 + V^2_{F,p}\Delta^2_{k,p,q}}}\right]~,
\end{align}

where $-\Lambda < k_0 < \Lambda$. From here, we can directly write down the $\log\mu$ derivative of the counter-term,

\begin{align}\nonumber
\frac{A^{' \mathrm{2L(a)}}_{1}({\bf k})}{\partial\log\mu}
		=
-\frac{N_f }{64 \pi^4\mu^2}\int \frac{\dd q_x\dd p_x}{(V_{F, k+q}+V_{F, p})(V_{F, k+q}+V_{F, p-q})}  
 \lambda^{\spmqty{1 & 5 \\  1 &  5};\spmqty{\alpha_1 & \alpha_3 \\ \sigma & \alpha_2}}_{\spmqty{k+q  & p-q \\ k & p }}
\lambda^{\spmqty{1 & 5 \\  1 &  5};\spmqty{\sigma & \alpha_2 \\ \alpha_1 & \alpha_3}}_{\spmqty{k  & p \\ k+q & p-q }}\times\\
	(ik_0+V_{F,k+q}\Delta_{k,p,q})\left[-\frac{\mu^2}{\mu ^2+\Delta_{k,p,q}^2 V_{F,k+q}^2}-\frac{\mu^2}{\mu ^2+\Delta_{k,p,q}^2 V_{F,p}^2}\right]~.
\end{align}

%%%%%%%%%%%%%%%%%%%%%%%%%%%%%%%%%%%%%%%%%%%%%%
%%%%%%%%%%%%%%%%%%%%%%%%%%%%%%%%%%%%%%%%%%%%%%

For $(N,M_1,M_2,M_3) = (1,1,5,5)$, we have from Eq.~\eqref{eq:2LoopFSEprime_b},

\begin{align}
{\bf \Sigma}^{' \mathrm{2L(b)}}_{1}({\bf k}) 
		=
-\frac{1}{4 \mu^2}
\int\dd {\bf q} \int \dd {\bf p} ~ 
\lambda^{\spmqty{1 & 5 \\  1 &  5};\spmqty{\alpha_1 & \alpha_3 \\ \sigma & \alpha_2}}_{\spmqty{k+q  & k+p \\ k & k+q+p }}
\lambda^{\spmqty{5 & 1 \\  1 &  5};\spmqty{\alpha_2 & \sigma \\ \alpha_1 & \alpha_3}}_{\spmqty{k+q+p  & k \\ k+q & k+p }}
	G_{1}({\bf k}+{\bf q})
	G_{5}({\bf k}+{\bf q}+{\bf p})
	G_{5}({\bf k}+{\bf p}) ~.
\end{align}

%with the explicit form of the fermion propagators, we have, 

%\begin{align}\nonumber
%{\bf \Sigma}^{' \mathrm{2L(b)}}_{1}({\bf k}) 
%		=
%-\frac{1}{4 \mu^2}
%\int \frac{\dd {\bf q}\dd {\bf p}}{V_{F, k+q}V_{F, k+q+p}V_{F, k+p}}  
%\lambda^{\spmqty{1 & 5 \\  1 &  5};\spmqty{\alpha_1 & \alpha_3 \\ \sigma & \alpha_2}}_{\spmqty{k+q  & k+p \\ k & k+q+p }}
%\lambda^{\spmqty{5 & 1 \\  1 &  5};\spmqty{\alpha_2 & \sigma \\ \alpha_1 & \alpha_3}}_{\spmqty{k+q+p  & k \\ k+q & k+p }}
%	\frac{1}{i(k_0+q_0)/V_{F, k+q}+v_{k+q}(k_x+q_x)+k_y+q_y}\times\\
%	\frac{1}{i(k_0+q_0+p_0)/V_{F, k+q+p}-v_{k+q+p}(k_x+q_x+p_x)-k_y - q_y - p_y}~
%	\frac{1}{i(k_0+p_0)/V_{F, k+p} -v_{k+p}(k_x+p_x)-k_y-p_y}~.
%\end{align}

Shifting $p\to p-k$, we have, 

\begin{align}
{\bf \Sigma}^{' \mathrm{2L(b)}}_{1}({\bf k}) 
		=
-\frac{1}{4 \mu^2}
\int\dd {\bf q} \int \dd {\bf p} ~ 
\lambda^{\spmqty{1 & 5 \\  1 &  5};\spmqty{\alpha_1 & \alpha_3 \\ \sigma & \alpha_2}}_{\spmqty{k+q  & p \\ k & q+p }}
\lambda^{\spmqty{5 & 1 \\  1 &  5};\spmqty{\alpha_2 & \sigma \\ \alpha_1 & \alpha_3}}_{\spmqty{q+p  & k \\ k+q & p }}
	G_{1}({\bf k}+{\bf q})
	G_{5}({\bf q}+{\bf p})
	G_{5}({\bf p}) ~.
\end{align}

\noindent Writing the Fermion propagators explicitly, and doing the partial fraction, we get,

\begin{align}\nonumber
{\bf \Sigma}^{' \mathrm{2L(b)}}_{1}({\bf k}) 
		=
-\frac{1}{4 \mu^2}\int\dd {\bf q} \int \dd {\bf p}~ \frac{1  }{V_{F, k+q}V_{F, p+q}V_{F,p}}
\lambda^{\spmqty{1 & 5 \\  1 &  5};\spmqty{\alpha_1 & \alpha_3 \\ \sigma & \alpha_2}}_{\spmqty{k+q  & p \\ k & q+p }}
\lambda^{\spmqty{5 & 1 \\  1 &  5};\spmqty{\alpha_2 & \sigma \\ \alpha_1 & \alpha_3}}_{\spmqty{q+p  & k \\ k+q & p }}\times\\\nonumber
	\frac{1}{i(k_0+q_0)/V_{F,k+q} + v_{k+q}(k_x+q_x) + k_y+q_y}\times\\\nonumber
	\left[\frac{1}{i(p_0+q_0)/V_{F,p+q} - v_{p+q}(p_x+q_x) - p_y-q_y} - \frac{1}{ip_0/V_{F,p}-v_pp_x-p_y}\right]\times\\
	\frac{1}{ip_0/V_{F,p}-i(p_0+q_0)/V_{F,p+q} - v_pp_x + v_{p+q}(p_x+q_x) + q_y}~.
\end{align}

First we integrate $p_y$, and then we do the partial fraction again, such that we get, 

\begin{align}\nonumber
{\bf \Sigma}^{' \mathrm{2L(b)}}_{1}({\bf k}) 
		=
-\frac{1}{4 \mu^2}\int\dd {\bf q} \int\frac{ \dd {p_0}\dd{p_x}}{8\pi^3}~ 
\lambda^{\spmqty{1 & 5 \\  1 &  5};\spmqty{\alpha_1 & \alpha_3 \\ \sigma & \alpha_2}}_{\spmqty{k+q  & p \\ k & q+p }}
\lambda^{\spmqty{5 & 1 \\  1 &  5};\spmqty{\alpha_2 & \sigma \\ \alpha_1 & \alpha_3}}_{\spmqty{q+p  & k \\ k+q & p }}\times
	\frac{i\pi({\rm sgn}[p_0]-{\rm sgn}[p_0+q_0])}{V_{F, k+q}V_{F, p+q}V_{F,p}}\times\\\nonumber
	\left[\frac{1}{i(k_0+q_0)/V_{F,k+q} + v_{k+q}(k_x+q_x) + k_y+q_y} - \frac{1}{ip_0/V_{F,p}-i(p_0+q_0)/V_{F,p+q} - v_pp_x + v_{p+q}(p_x+q_x) + q_y}\right]\times\\
	\frac{1}{ip_0(V^{-1}_{F,p}-V^{-1}_{F,p+q})-iq_0(V^{-1}_{F,k+q}+V^{-1}_{F,p+q})-ik_0V^{-1}_{F,k+q}+v_{p+q}(p_x+q_x)-v_{k+q}(k_x+q_x)-v_pp_x-k_y}~.
\end{align}

Integrating $q_y$, we get, 

\begin{align}\nonumber
{\bf \Sigma}^{' \mathrm{2L(b)}}_{1}({\bf k}) 
		=
-\frac{1}{4 \mu^2}\int\frac{\dd {q_0}\dd{q_x}  \dd {p_0}\dd{p_x}}{64\pi^6}~ 
\lambda^{\spmqty{1 & 5 \\  1 &  5};\spmqty{\alpha_1 & \alpha_3 \\ \sigma & \alpha_2}}_{\spmqty{k+q  & p \\ k & q+p }}
\lambda^{\spmqty{5 & 1 \\  1 &  5};\spmqty{\alpha_2 & \sigma \\ \alpha_1 & \alpha_3}}_{\spmqty{q+p  & k \\ k+q & p }}\times
	\frac{i\pi({\rm sgn}[p_0]-{\rm sgn}[p_0+q_0])}{V_{F, k+q}V_{F, p+q}V_{F,p}}\times\\
	\frac{-i\pi({\rm sgn}[k_0+q_0]-{\rm sgn}[p_0(V^{-1}_{F,p}-V^{-1}_{F,p+q})-q_0V^{-1}_{F,p+q}])}{ip_0(V^{-1}_{F,p}-V^{-1}_{F,p+q})-iq_0(V^{-1}_{F,k+q}+V^{-1}_{F,p+q})-ik_0V^{-1}_{F,k+q}+v_{p+q}(p_x+q_x)-v_{k+q}(k_x+q_x)-v_pp_x-k_y}~.
\end{align}

Finally integrating $q_0$ and $p_0$ and simplifying, we obtain,

\begin{align}\nonumber
{\bf \Sigma}^{' \mathrm{2L(b)}}_{1}({\bf k}) 
		=
-\frac{1}{64 \pi^4\mu^2}\int \frac{\dd q_x\dd p_x}{(V_{F, k+q}+V_{F, p})(V_{F, k+q}+V_{F, p-q})}  
\lambda^{\spmqty{1 & 5 \\  1 &  5};\spmqty{\alpha_1 & \alpha_3 \\ \sigma & \alpha_2}}_{\spmqty{k+q  & p \\ k & q+p }}
\lambda^{\spmqty{5 & 1 \\  1 &  5};\spmqty{\alpha_2 & \sigma \\ \alpha_1 & \alpha_3}}_{\spmqty{q+p  & k \\ k+q & p }}\times\\
	(ik_0+V_{F,k+q}\Delta^{\prime}_{k,p,q})\log\left[\frac{\Lambda}{\sqrt{k_0^2 + V^2_{F,k+q}{\Delta^{\prime}}^2_{k,p,q}}\sqrt{k_0^2 + V^2_{F,p}{\Delta^{\prime}}^2_{k,p,q}}}\right]~,
\end{align}

where, 
\begin{align}
\Delta^{\prime}_{k,p,q} = -(v_{p+q}-v_p)p_x - (v_{p+q}-v_{k+q})q_x + (v_{k+q}-v_k)k_x + \varepsilon_1({\vec k},v_k)~.
\end{align}

The $\log\mu$ derivative of the counter-term is given as,

\begin{align}\nonumber
\frac{A^{' \mathrm{2L(b)}}_{1}({\bf k})}{\partial\log\mu}
		=
\frac{1}{64 \pi^4\mu^2}\int \frac{\dd q_x\dd p_x}{(V_{F, k+q}+V_{F, p})(V_{F, k+q}+V_{F, p-q})}  
\lambda^{\spmqty{1 & 5 \\  1 &  5};\spmqty{\alpha_1 & \alpha_3 \\ \sigma & \alpha_2}}_{\spmqty{k+q  & p \\ k & q+p }}
\lambda^{\spmqty{5 & 1 \\  1 &  5};\spmqty{\alpha_2 & \sigma \\ \alpha_1 & \alpha_3}}_{\spmqty{q+p  & k \\ k+q & p }}\times\\
	(ik_0+V_{F,k+q}\Delta^{\prime}_{k,p,q})\left[-\frac{\mu^2}{\mu^2 + V^2_{F,k+q}{\Delta^{\prime}}^2_{k,p,q}} -\frac{\mu^2}{\mu^2 + V^2_{F,p}{\Delta^{\prime}}^2_{k,p,q}}\right]~.
\end{align}

For $(N,M_1,M_2,M_3) = (1,1,5,5)$, we have from Eq.~\eqref{eq:2LoopFSEprime_c},

\begin{align}
{\bf \Sigma}^{' \mathrm{2L(c)}}_{1}({\bf k}) 
		=
-\frac{1}{4 \mu^2}
\int\dd {\bf q} \int \dd {\bf p}~ \lambda^{\spmqty{1 & 1\\  1 &  5};\spmqty{\alpha_1 & \sigma \\ \sigma & \alpha_3}}_{\spmqty{k+q  & k \\ k & k+q }}
\lambda^{\spmqty{5 & 5 \\  1 &  1};\spmqty{\alpha_2 & \alpha_3 \\ \alpha_1 & \alpha_2}}_{\spmqty{k+q+p  & k+q \\ k+q & k+p+q }}
	G_{1}({\bf k}+{\bf q})
	G_{5}({\bf k}+{\bf q}+{\bf p})
	G_{5}({\bf k}+{\bf q}) ~.
\end{align}

Shifting $q\to q-k$, and explicitly expressing the fermion propagators, we have, 

\begin{align}\nonumber
{\bf \Sigma}^{' \mathrm{2L(c)}}_{1}({\bf k}) 
		=
-\frac{1}{4 \mu^2}
\int\frac{\dd {\bf q}}{V^2_{F,q}} \int \frac{\dd {\bf p}}{V_{F,p+q}}~ \lambda^{\spmqty{1 & 1 \\  1 &  5};\spmqty{\alpha_1 & \sigma \\ \sigma & \alpha_3}}_{\spmqty{q  & k \\ k & q }}
\lambda^{\spmqty{5 & 5 \\  1 &  1};\spmqty{\alpha_2 & \alpha_3 \\ \alpha_1 & \alpha_2}}_{\spmqty{q+p  & q \\ q & p+q }}
	\frac{1}{iq_0 V^{-1}_{F,q} + v_qq_x + q_y}~\frac{1}{iq_0 V^{-1}_{F,q} - v_qq_x - q_y}\times\\
	\frac{1}{i(p_0+q_0) V^{-1}_{F,p+q} - v_{p+q}(p_x+q_x) - p_y - q_y} ~.
\end{align}

Integrating $p_y$ first yields a factor $-i\pi{\rm sgn}(p_0+q_0)$. Afterwards, we can integrate $q_y$ and simplify such that,

\begin{align}
{\bf \Sigma}^{' \mathrm{2L(c)}}_{1}({\bf k}) 
		=
\frac{1}{4 \mu^2}
\int\frac{\dd q_0\dd q_x\dd p_0\dd p_x }{64\pi^4V_{F,q}V_{F,p+q}}~ \lambda^{\spmqty{1 & 1 \\  1 &  5};\spmqty{\alpha_1 & \sigma \\ \sigma & \alpha_3}}_{\spmqty{q  & k \\ k & q }}
\lambda^{\spmqty{5 & 5 \\  1 &  1};\spmqty{\alpha_2 & \alpha_3 \\ \alpha_1 & \alpha_2}}_{\spmqty{q+p  & q \\ q & p+q }}
	~\frac{{\rm sgn}(p_0+q_0){\rm sgn}(q_0)}{q_0} ~.
\end{align}

which vanishes after $p_0$, $q_0$ integration.

\subsubsection{Involving hot spots $1$, $5$, $4$ and $8$}

The non-nested channels are expected to contribute near hot-spots regime only. Since the weight of the four fermion coupling is mostly centered in the region $\approx \mu/v$, it does not discriminate significantly between the nested and the non-nested channels, as far as the feedback to the self-energy is concerned. We explicitly show this for the following case. 
Consider $(N,M_1,M_2,M_3) = (1,8,4,5)$, we have from Eq.~\eqref{eq:2LoopFSEprime_a},

\begin{align}
{\bf \Sigma}^{' \mathrm{2L(a)}}_{1}({\bf k}) 
		=
\frac{N_f}{4 \mu^2}
\int\dd {\bf q} \int \dd {\bf p} ~ 
 \lambda^{\spmqty{4 & 8 \\  1 &  5};\spmqty{\alpha_1 & \alpha_3 \\ \sigma & \alpha_2}}_{\spmqty{k+q  & p-q \\ k & p }}
\lambda^{\spmqty{1 & 5 \\  4 &  8};\spmqty{\sigma & \alpha_2 \\ \alpha_1 & \alpha_3}}_{\spmqty{k  & p \\ k+q & p-q }}
	G_{4}({\bf k}+{\bf q})
	G_{5}({\bf p})
	G_{8}({\bf p}-{\bf q}) ~,
\end{align}

with the explicit form of the fermion propagators, we have, 

\begin{align}\nonumber
{\bf \Sigma}^{' \mathrm{2L(a)}}_{1}({\bf k}) 
		=
\frac{N_f}{4 \mu^2}
\int \frac{\dd {\bf q}\dd {\bf p}}{V_{F, k+q}V_{F, p}V_{F, p-q}}  
\lambda^{\spmqty{4 & 8 \\  1 &  5};\spmqty{\alpha_1 & \alpha_3 \\ \sigma & \alpha_2}}_{\spmqty{k+q  & p-q \\ k & p }}
\lambda^{\spmqty{1 & 5 \\  4 &  8};\spmqty{\sigma & \alpha_2 \\ \alpha_1 & \alpha_3}}_{\spmqty{k  & p \\ k+q & p-q }}
	\frac{1}{i(k_0+q_0)/V_{F, k+q}+v_{k+q}(k_x+q_x)-k_y-q_y}\times\\
	\frac{1}{ip_0/V_{F, p}-v_{p}p_x-p_y}~
	\frac{1}{i(p_0-q_0)/V_{F, p-q} -v_{p-q}(p_x-q_x)+p_y-q_y}~.
\end{align}

Integrating $p_y$ first, we get,

\begin{align}\nonumber
{\bf \Sigma}^{' \mathrm{2L(a)}}_{1}({\bf k}) 
		=
\frac{N_f}{4 \mu^2}
\int \frac{\dd {\bf q}\dd p_x \dd p_0}{8\pi^3V_{F, k+q}V_{F, p}V_{F, p-q}}  
\lambda^{\spmqty{4 & 8 \\  1 &  5};\spmqty{\alpha_1 & \alpha_3 \\ \sigma & \alpha_2}}_{\spmqty{k+q  & p-q \\ k & p }}
\lambda^{\spmqty{1 & 5 \\  4 &  8};\spmqty{\sigma & \alpha_2 \\ \alpha_1 & \alpha_3}}_{\spmqty{k  & p \\ k+q & p-q }}
\frac{1}{i(k_0+q_0)V^{-1}_{F, k+q}+v_{k+q}(k_x+q_x)-k_y-q_y}\times\\
	\frac{-i\pi\left[{\rm sgn}(p_0-q_0) + {\rm sgn}(p_0)\right]}{ip_0\left(V^{-1}_{F,p-q} + V^{-1}_{F,p}\right) - v_{p-q}(p_x-q_x) - q_y
	- v_pp_x - iq_0 V^{-1}_{F,p-q}}~.
\end{align}

Now, integrating $q_y$ and simplifying the resulting expression, we obtain,
\begin{align}\nonumber
{\bf \Sigma}^{' \mathrm{2L(a)}}_{1}({\bf k}) 
		=
-\frac{N_f}{4 \mu^2}
\int \frac{\dd q_x \dd q_0\dd p_x \dd p_0}{64\pi^4V_{F, k+q}V_{F, p}V_{F, p-q}}  
\lambda^{\spmqty{4 & 8 \\  1 &  5};\spmqty{\alpha_1 & \alpha_3 \\ \sigma & \alpha_2}}_{\spmqty{k+q  & p-q \\ k & p }}
\lambda^{\spmqty{1 & 5 \\  4 &  8};\spmqty{\sigma & \alpha_2 \\ \alpha_1 & \alpha_3}}_{\spmqty{k  & p \\ k+q & p-q }}
\times\\
	\frac{\left[{\rm sgn}(p_0-q_0) + {\rm sgn}(p_0)\right]\left[{\rm sgn}(k_0+q_0) - {\rm sgn}\left(p_0+p_0V_{F,p-q}V^{-1}_{F,p} - q_0\right)\right]}{ip_0\left(V^{-1}_{F,p-q} + V^{-1}_{F,p}\right) - iq_0\left(V^{-1}_{F,k+q} + V^{-1}_{F,p-q}\right) - ik_0 V^{-1}_{F,k+q} - \Delta^{\prime\prime}_{k,p,q}}~,
\end{align}
where, 
\begin{align}
 \Delta^{\prime\prime}_{k,p,q} = (v_{k+q}-v_{p-q})q_x + (v_{p-q}+v_p)p_x + (v_{k+q}-v_k)k_x + \varepsilon_4({\vec k},v_k)~.
\end{align}
{\color{red}\noindent Next, doing the $p_0 ~(|p_0| < \Lambda)$ integration followed by $q_0 ~(|q_0| < \Lambda)$ integration and keeping the dominant contribution, we get,

\begin{align}\nonumber
{\bf \Sigma}^{' \mathrm{2L(a)}}_{1}({\bf k}) 
		=
\frac{N_f }{64 \pi^4\mu^2}\int \frac{\dd q_x\dd p_x}{(V_{F, p-q}+V_{F, p})(V_{F, k+q}-V_{F, p})(V_{F, k+q}+V_{F, p-q})}  
 \lambda^{\spmqty{1 & 5 \\  1 &  5};\spmqty{\alpha_1 & \alpha_3 \\ \sigma & \alpha_2}}_{\spmqty{k+q  & p-q \\ k & p }}
\lambda^{\spmqty{1 & 5 \\  1 &  5};\spmqty{\sigma & \alpha_2 \\ \alpha_1 & \alpha_3}}_{\spmqty{k  & p \\ k+q & p-q }}\times\\
	\Bigg[-(V_{F, p-q}+V_{F, p}) (\Delta^{\prime\prime}_{k,p,q} V_{F, k+q}+i k_0) \log \left(\frac{\sqrt{k_0^2+\Delta^{\prime\prime}_{k,p,q}^2 V_{F, k+q}^2}}{\Lambda }\right) \\\nonumber
	+(V_{F, k+q}-V_{F, p}) (ik_0- \Delta^{\prime\prime}_{k,p,q} V_{F, p-q}) \log \left(\frac{\sqrt{k_0^2+\Delta^{\prime\prime}_{k,p,q}^2 V_{F, p-q}^2}}{\Lambda }\right) \\
	+(V_{F, k+q}+V_{F, p-q}) (\Delta^{\prime\prime}_{k,p,q} V_{F, p}+i k_0) \log \left(\frac{\sqrt{k_0^2+\Delta^{\prime\prime}_{k,p,q}^2 V_{F, p}^2}}{\Lambda }\right)~\Bigg].
\end{align}}
