# Supplementary material for: Field-theoretic functional renormalization group formalism for non-Fermi liquids and its application to the antiferromagnetic quantum critical metal in two dimensions
Source: arXiv:2208.00730 source file (2023-01-06)
Supplement: Supplementary file 5 [file appendixquasifixed.tex]

\section{Quasi-Fixed Point of the Four-Fermion Beta Function}
\label{sec:quasifixed}

In this appendix we will calculate and describe the properties of the non-Hermitian, quasi-fixed point obtained from the solution of the shifted, four-fermion coupling beta function for the Group I-2 pairing channels  in Eq. \eqref{eq:betaallwaves_main0}. We consider a UV theory in which all coupling functions are independent of momentum and the four-fermion coupling is zero at the UV cutoff energy scale, as in Eq. \eqref{eq:allIncond}.

To find the flow of the four-fermion coupling under this considerations, we need to project Eq. \eqref{eq:betaallwaves_matrix} into a space we can visualize. In order to do that, we need to write $\tilde{\lambda}$ from the aforementioned equation in a basis
\begin{equation}
\tilde{\lambda}^{(n)}(\ell) = \sum_{j = 0}^{\infty}c_{j,n}(\ell)\tilde{\lambda}^{(n),(j)},
\end{equation}
where $\tilde{\lambda}^{(n)}_{QK} = \tilde{\lambda}^{(n)}_{2PP \spmqty{Q & -Q \\ K & -K}}$ with $n = (-,d), (+,s)$ represent the four-fermion coupling. $\tilde{\lambda}^{(n),(j)}_{QK}$ represent an element of an ``orthonormal basis'' and the coefficients $c_{j,n}(\ell)$ contain all the $\ell$-dependence. Assuming that the basis elements are normalized, we can project on any state by means of the ``matrix'' multiplication
\begin{equation}
(AB)_{KP} = \int\frac{\dd Q}{2\pi\Lambda}A_{KQ}B_{QP},
\end{equation}
where the norm squared is naturally defined as
\begin{equation}
\lVert A \rVert^2 = \tr{AA} =  \int\frac{\dd K \dd P}{(2\pi\Lambda)^2}A_{KP}A_{PK},
\end{equation}
and the basis elements satisfy
\begin{equation}
\int\frac{\dd K \dd P}{(2\pi\Lambda)^2}\tilde{\lambda}^{(n),(i)}_{KP}\tilde{\lambda}^{(n),(j)}_{PK} = \delta_{ij}.
\end{equation}
The beta function on this language is just
\begin{equation}
\frac{\partial\tilde{\lambda}^{(n)}(\ell)}{\partial\ell} = \sum_{j = 0}^{\infty}\frac{\partial c_{j,n}(\ell)}{\partial\ell}\tilde{\lambda}^{(n),(j)}.
\end{equation}

To be precise, 
%let us consider $n = (-,d)$. Also, 
let us use the following notation $t(\ell) = c_{0,n}(\ell)$ so that
\begin{equation}
\tilde{\lambda}^{(n)}(\ell) = t(\ell)\tilde{\lambda}^{(n),(0)} + \sum_{j = 1}^{\infty}c_{j,n}(\ell)\tilde{\lambda}^{(n),(j)},
\label{eq:lambdaexpansion}
\end{equation}
and
\begin{equation}
\frac{\partial\tilde{\lambda}^{(n)}(\ell)}{\partial\ell} = \frac{\partial t(\ell)}{\partial\ell}\tilde{\lambda}^{(n),(0)} + \sum_{j = 1}^{\infty}\frac{\partial c_{j,n}(\ell)}{\partial\ell}\tilde{\lambda}^{(n),(j)}.
\end{equation}

In principle, we do not know whether or not we can choose a completely orthonormal basis to write the four-fermion coupling, such that the projection doesn't mix the (projected) flow on $t(\ell)$ with the (projected) flow on the rest of the $c_{j>1,n}(\ell)$. This can happen if we choose an anzats for $\tilde{\lambda}^{(n),(0)}$ with a momentum profile that allows the second term in Eq. \eqref{eq:lambda_exp} to be non-positive. This just means that the projection plane determined by $t(\ell)$ and the other $c_{j,n}(\ell)$s is mixing non-Hermiatian channels with (Hermitian) channels that reach the real fixed point faster. Fortunately, we do not have to choose a full basis, just the first element $\tilde{\lambda}^{(n),(0)}$. The choice, needs to maximize the non-Hermitian expectation value of Eq. \eqref{eq:lambda_fp_eq}, so that we can approximate $c_{j>1,n}(\ell) = 0, \partial c_{j>1,n}(\ell) / \partial\ell = 0$ and perform the projection
\begin{equation}
\frac{\partial t(\ell)}{\partial\ell} = \tr{\frac{\partial\tilde{\lambda}^{(n)}(\ell)}{\partial\ell}\tilde{\lambda}^{(n),(0)}} = \int\frac{\dd K \dd P}{(2\pi\Lambda)^2}\frac{\partial\tilde{\lambda}^{(n)}_{KP}(\ell)}{\partial\ell}\tilde{\lambda}^{(n),(0)}_{PK}.
\label{eq:tproj}
\end{equation}
With this equation, we can probe the flow of $\tilde{\lambda}^{(n)}$ by exploring the flow of $t(\ell)$, which is a scalar quantity that only depends on the length scale $\ell$. This is because, with the right choice of $\tilde{\lambda}^{(n),(0)}$ we can consider the right hand side of the previous equation to represent a (approximate) beta function for $t(\ell)$, $-\beta^{(z)}$, where all the momentum contributions have been summed over, i.e.
\begin{equation}
\frac{\partial t(\ell)}{\partial\ell} \approx -\beta^{(t)}.
\label{eq:betat}
\end{equation}

Now that we now the constraints of we need to impose to our analysis, we start by considering a $\ell_0 \gg 1$ and $0 < \ell \ll \ell_0$. In this region we have a (very) slow-varying, small nesting angle $v_0(\ell)$. Therefore, we can fix $v_0(\ell) \approx v_0(0)$ for some large value of $\ell_0$. Secondly, as mentioned above, we need a non-Hermitian solution for the expectation value of the beta function. Fortunately, we already have a solution in Eq. \eqref{eq:betaallwaves_matrix} and the vector $f_K$ of Eq. \eqref{eq:fvector}, solution of the equation $ \left( \frac{I}{2}  + L^\dagger + H \right) f = 0$. This function can be used to construct a $\tilde{\lambda}^{(n),(0)}$ with the appropriate momentum profile to get the UV theory needed to reconstruct the quasi-fixed points at low energies.
%As it turns out, this vector $f$ is the precise function we need to extract the quasi-fixed point from the full beta function as it results in a non-Hermitian fixed point in Eq. \eqref{eq:lambda_exp}.

In order to obtain a graphic representation of the no-Hermitian fixed points, we need to impose an approximation to $f_K$, as the normalization factor in Eq. \eqref{eq:fvector} does not tame the highly divergent nature of $\sqrt{1/\abs{K}}$ in the IR limit, which could be troublesome for obtaining controlled numerics on the plting of the fixed points.
%After discarding the $c_{j>1,n}(\ell)$ terms, 
The solution is to impose cutoffs in our anzats $f_K$, via a product of Heaviside functions
\begin{equation}
f_K = \sqrt{\frac{\Lambda}{\abs{K}}}\Theta(\abs{K}-\varepsilon)\Theta(\Delta -\abs{K}).
\end{equation}
We choose $\Delta$ to be a UV momentum cutoff of the order of the momentum cutoff $\Lambda$ and $0 < \varepsilon \ll \Lambda$ the IR momentum cutoff. We can further simplify by introducing the bra-ket notation
\begin{equation}
\langle f | f \rangle = \int\frac{\dd K}{2\pi\Lambda}f_K f_K = \frac{1}{2\pi} \log\left(\frac{\Delta}{\varepsilon}\right).
\label{eq:braketnotation}
\end{equation}
After discarding the $c_{j>1,n}(\ell)$ terms, we can write Eq. \eqref{eq:lambdaexpansion} as
\begin{equation}
\tilde{\lambda}^{(n)}_{KP}(\ell) = t(\ell)\frac{f_K f_P}{\langle f | f \rangle},
\label{eq:lambdatf}
\end{equation}
where 
\begin{equation}
\tilde{\lambda}^{(n),(0)}_{KP} = \frac{f_K f_P}{\langle f | f \rangle}.
\end{equation}
%with
%\begin{equation}
%\langle f | f \rangle^2 = \int\frac{\dd K \dd P}{(2\pi \Lambda)^2}f_K f_P f_K f_P = \left(\frac{1}{2\pi} \log\left(\frac{\Delta}{\varepsilon}\right)\right)^2.
%\end{equation}

With these equation we can write the projection in Eq. \eqref{eq:tproj} as
\begin{equation}
\langle f | f\rangle\frac{\partial t(\ell)}{\partial\ell} = \langle f | \frac{\partial\tilde{\lambda}^{(n)}(\ell)}{\partial\ell} | f \rangle = \int\frac{\dd K \dd P}{(2\pi\Lambda)^2}f_K \frac{\partial\tilde{\lambda}^{(n)}_{KP}(\ell)}{\partial\ell} f_P.
\label{eq:tfproj}
\end{equation}
Then, we can rewrite Eq. \eqref{eq:betaallwaves_main0} sandwiched by $f$ as
\begin{equation}
\begin{aligned} 
\langle f |\frac{\partial }{\partial\ell}\tilde{\lambda}^{(n)} | f \rangle = 
 & -\int\frac{\dd P \dd K}{(2\pi\Lambda)^2}f_P\left(1 + K\frac{\partial}{\partial K} + P\frac{\partial}{\partial P} 
  + \hat \eta_K + \hat \eta_P 
\right)
 \tilde{\lambda}^{(n)}_{PK}f_K
 \\ & 
   -\frac{1}{4\pi} \int \frac{\dd P \dd Q \dd K}{(2\pi\Lambda)^3}
f_P \tilde{\lambda}^{(n)}_{PQ} 
 \tilde{\lambda}^{(n)}_{QK} f_K- \frac{2}{N_f}
Y_{PP}^{(\pm)} 
1^{\spmqty{s \\ d}}
\int\frac{\dd P \dd K}{(2\pi\Lambda)^2}f_P R(P, K ) f_K.
\end{aligned}
\label{eq:betafullf}
\end{equation}
The derivative terms can be expanded as
\begin{equation}
K\partial_K f_K = -\frac{1}{2}f_K + \sqrt{\varepsilon\Lambda}\delta(\abs{K}-\varepsilon) - \sqrt{\Delta\Lambda}\delta(\Delta - \abs{K}).
\end{equation}
The boundary terms dependnon the definition of the delta function inside the interval. However, if we include them inside the interval $[\varepsilon,\Delta]$ they cancel in the integration $\int
(K\partial_K f_K)f_K$. Otherwise, we can work in the open interval $(\varepsilon,\Delta)$, which means that the contribution for the zero measure set of the boundary points is negligible. With this, and with Eq. \eqref{eq:lambdatf}, equation \eqref{eq:betafullf} is
\begin{equation}
\begin{aligned} 
\frac{\partial t(\ell)}{\partial\ell} = \frac{\langle f |\frac{\partial }{\partial\ell}\tilde{\lambda}^{(n)} | f \rangle}{\langle f | f\rangle} = & - \left[
%\frac{1}{4\pi}
% \langle f | f \rangle^2 
 \frac{1}{4\pi} t(\ell)^2 + 2 \frac{\langle f | \hat{\eta} | f \rangle}{\langle f | f \rangle} t(\ell) + \frac{2}{N_f}
Y_{PP}^{(\pm)} 1^{\spmqty{s \\ d}}\frac{\langle f | R | f \rangle}{\langle f | f \rangle}\right].
\end{aligned}
\label{eq:betatpolynomial}
\end{equation}
The quantities in bra-kets can be easily calculated. They are
\begin{align}
\langle f | \hat{\eta} | f \rangle = & \frac{(N_c^2 - 1)v}{4\pi N_c N_f c}\frac{\log\left(\frac{\Lambda}{2 v c \varepsilon}\right)}{2\pi} 
+ 2\left\langle f \left| \hat{\eta}^{(2)} \right| f \right\rangle
% - (z-1)\left\langle f | f \right\rangle, 
\label{eq:etaevf}
\\ \langle f | R | f \rangle = & \frac{v}{4 \pi c}\log\left(\frac{2}{v}\right),
\label{eq:Revf}
\end{align}
where $c = c(v_0)$ and in the second calculation, the first integral is solved taking the limits $\varepsilon \to 0$ and $\Delta \to \infty$. The expression for $\eta^{(2)}$ is given by Eq. \eqref{eq:eta_prime} and is of order $\lambda^2$, i.e. of order $t(\ell)^2$. 
%Therefore, to first order in $w$
%\begin{equation}
%z - 1 = \frac{N_c^2 - 1}{2\pi N_c N_f}\left[1 - \frac{2}{\pi}\log\left(\frac{1}{c}\right)\right]\frac{v}{c}.
%\label{eq:zedfeq}
%\end{equation}
%and
%, according with Eq. \eqref{eq:eta2_estimation}
%\begin{equation}
%\left\langle f \left| \hat{\eta}^{(2)} \right| f \right\rangle \sim \frac{\pi^2 v}{4 c}\int_{\varepsilon}^{\Delta}\frac{\dd K}{2\pi \Lambda}f_K\frac{\Lambda}{\Lambda + c v\abs{K}}f_K = \frac{\pi v}{8 c}\log\left(\frac{\Lambda}{c v \varepsilon}\right),
%\end{equation}
%where we have taken the $\Delta \to \infty$ and $\varepsilon \to 0$ limits again. In summary, the explicit value of Eq. \eqref{eq:etaevf} is
Now, according to Eq. \eqref{eq:eta_prime}
\begin{equation}
\begin{aligned}
\left\langle f \left| \hat{\eta}^{(2)} \right| f \right\rangle = & \frac{N_f}{8^2\pi^2}\int_\varepsilon^\Delta \frac{\dd K \dd L }{(2\pi\Lambda)^2} \int \frac{\dd P \dd Q}{(2\pi\Lambda)^2}f_K \hat{\lambda}^{\spmqty{1 & 5 \\ 1 & 5};\spmqty{\alpha_1 & \alpha_3 \\ \sigma & \alpha_2}}_{\spmqty{L+Q & P-Q  \\ L & P}} \hat{\lambda}^{\spmqty{1 & 5 \\ 1 & 5};\spmqty{\sigma & \alpha_2 \\ \alpha_1 & \alpha_3}}_{\spmqty{L & P \\ L+Q & P-Q}}2\pi\Lambda \delta(K - L)f_L.
\end{aligned}
\label{eq:etavfprelim}
\end{equation}
We only include the first term since we are turning off all hot spot channels that are not part of the $2PP$ pairing channel in Group I-2. From Eqs. \eqref{eq:tildelambda0} and \eqref{eq:propmatrix} we can write
\begin{align}
&\begin{aligned}
\hat{\lambda}^{\spmqty{1 & 5 \\ 1 & 5};\spmqty{\alpha_1 & \alpha_3 \\ \sigma & \alpha_2}}_{\spmqty{L+Q & P-Q  \\ L & P}} = & \frac{\sqrt[4]{\hat{V}_{F,L+Q}\hat{V}_{F,P-Q}\hat{V}_{F,L}\hat{V}_{F,P}}}{2}\left[\mathsf{S}^{\alpha_1 , \alpha_3}_{\sigma , \alpha_2}\left(\tilde{\lambda}^{(+);(s)}_{\spmqty{L+Q & P-Q  \\ L & P}} + \tilde{\lambda}^{(+);(d)}_{\spmqty{L+Q & P-Q  \\ L & P}}\right)\right.
\\ & \left. + \mathsf{A}^{\alpha_1 , \alpha_3}_{\sigma , \alpha_2}\left(\tilde{\lambda}^{(-);(s)}_{\spmqty{L+Q & P-Q  \\ L & P}} + \tilde{\lambda}^{(-);(d)}_{\spmqty{L+Q & P-Q  \\ L & P}}\right)\right],
\end{aligned}
\\ &\begin{aligned}
\hat{\lambda}^{\spmqty{1 & 5 \\ 1 & 5};\spmqty{\sigma & \alpha_2 \\ \alpha_1 & \alpha_3}}_{\spmqty{L & P \\ L+Q & P-Q}} = & \frac{\sqrt[4]{\hat{V}_{F,L+Q}\hat{V}_{F,P-Q}\hat{V}_{F,L}\hat{V}_{F,P}}}{2}\left[\mathsf{S}^{\sigma , \alpha_2}_{\alpha_1 , \alpha_3}\left(\tilde{\lambda}^{(+);(s)}_{\spmqty{L & P \\ L+Q & P-Q}} + \tilde{\lambda}^{(+);(d)}_{\spmqty{L & P \\ L+Q & P-Q}}\right)\right.
\\ & \left. + \mathsf{A}^{\sigma , \alpha_2}_{\alpha_1 , \alpha_3}\left(\tilde{\lambda}^{(-);(s)}_{\spmqty{L & P \\ L+Q & P-Q}} + \tilde{\lambda}^{(-);(d)}_{\spmqty{L+Q & P-Q  \\ L & P}}\right)\right].
\end{aligned}
\end{align}
With this identities, we can rewrite the argument of Eq. \eqref{eq:etavfprelim} as
\begin{equation}
\begin{aligned}
\hat{\lambda}^{\spmqty{1 & 5 \\ 1 & 5};\spmqty{\alpha_1 & \alpha_3 \\ \sigma & \alpha_2}}_{\spmqty{L+Q & P-Q  \\ L & P}} \hat{\lambda}^{\spmqty{1 & 5 \\ 1 & 5};\spmqty{\sigma & \alpha_2 \\ \alpha_1 & \alpha_3}}_{\spmqty{L & P \\ L+Q & P-Q}} = & \frac{\sqrt{\hat{V}_{F,L+Q}\hat{V}_{F,P-Q}\hat{V}_{F,L}\hat{V}_{F,P}}}{8}\times
\\ &\left[ \left(\tilde{\lambda}^{(+);(s)}_{\spmqty{L+Q & P-Q  \\ L & P}} + \tilde{\lambda}^{(+);(d)}_{\spmqty{L+Q & P-Q  \\ L & P}}\right)\left(\tilde{\lambda}^{(+);(s)}_{\spmqty{L & P \\ L+Q & P-Q}} + \tilde{\lambda}^{(+);(d)}_{\spmqty{L & P \\ L+Q & P-Q}}\right) \right.
\\ & \left. + \left(\tilde{\lambda}^{(-);(s)}_{\spmqty{L+Q & P-Q  \\ L & P}} + \tilde{\lambda}^{(-);(d)}_{\spmqty{L+Q & P-Q  \\ L & P}}\right)\left(\tilde{\lambda}^{(-);(s)}_{\spmqty{L & P \\ L+Q & P-Q}} + \tilde{\lambda}^{(-);(d)}_{\spmqty{L+Q & P-Q  \\ L & P}}\right) \right].
\end{aligned}
\end{equation}
Below we will only consider one channel, so let us take the example of turning off all interactions except $(-,d)$. Furthermore, recall that we are considering a theory with UV coupling functions independent of momentum, let us approximate $V_F \sim 1$ so that
\begin{equation}
\begin{aligned}
\frac{\left\langle f \left| \hat{\eta}^{(2)} \right| f \right\rangle}{\left\langle f | f \right\rangle} = & \frac{N_f}{8^3\pi^2}\int_\varepsilon^\Delta \frac{\dd K \dd L }{(2\pi\Lambda)^2} \int \frac{\dd P \dd Q}{(2\pi\Lambda)^2}\frac{f_K f_L}{\left\langle f | f \right\rangle} \tilde{\lambda}^{(-);(d)}_{\spmqty{L+Q & P-Q  \\ L & P}} \tilde{\lambda}^{(-);(d)}_{\spmqty{L & P \\ L+Q & P-Q}}2\pi\Lambda \delta(K - L)
\\ = & \frac{N_f}{8^3\pi^2} t(\ell)^2\int_\varepsilon^\Delta \frac{\dd K \dd L }{(2\pi\Lambda)^2} \int \frac{\dd P \dd Q}{(2\pi\Lambda)^2}\tilde{\lambda}^{(-);(d),(0)}_{\spmqty{K & -K \\ L & -L}} \tilde{\lambda}^{(-);(d),(0)}_{\spmqty{L+Q & P-Q  \\ L & P}} \tilde{\lambda}^{(-);(d),(0)}_{\spmqty{L & P \\ L+Q & P-Q}}2\pi\Lambda \delta(K - L)
\\ = & \frac{N_f}{8^3\pi^2} t(\ell)^2\int_\varepsilon^\Delta \frac{\dd K }{2\pi\Lambda} \int \frac{\dd P \dd Q}{(2\pi\Lambda)^2}\tilde{\lambda}^{(-);(d),(0)}_{\spmqty{K & -K \\ K & -K}} \tilde{\lambda}^{(-);(d),(0)}_{\spmqty{K+Q & P-Q  \\ K & P}} \tilde{\lambda}^{(-);(d),(0)}_{\spmqty{K & P \\ K+Q & P-Q}}.
\end{aligned}
\label{eq:etavfprelim2}
\end{equation}
The momentum dependence on the couplings restrict us from using Eq. \eqref{eq:lambdatf} directly. Regardless, the dependence on $\tilde{\lambda}$ of this expectation value clearly means that this quantity is proportional to $t(\ell)^2$ and to $w^3$, the latter due to the fact that the integral of $\tilde{\lambda}$ is proportional to $w$ near the quasi-fixed points and the bottleneck, according to the discussion between Eqs. \eqref{eq:betaallwaves_matrix}-\eqref{eq:lambda_exp}. Since this would only produce sub-leading terms of order $w^3$ and $w^{3/2}$ in the roots of Eq. \eqref{eq:betatpolynomial}, we can drop the $\eta^{(2)}$-term from Eq. \eqref{eq:etaevf} to obtain
\begin{equation}
\langle f | \hat{\eta} | f \rangle = \frac{N_c^2 - 1}{8\pi^2 N_c N_f}\frac{v}{c} \log\left(\frac{\Lambda}{2 v c \varepsilon}\right).
%+ \frac{N_c^2 - 1}{4\pi^2 N_c N_f}\log\left(\frac{\Delta}{\varepsilon}\right)\left[\frac{2}{\pi}\log\left(\frac{1}{c}\right) - 1\right]\frac{v}{c}.
\label{eq:etaevfexplicit}
\end{equation}

%According to Eq. \eqref{eq:lambda_fixedpt_largekp}, in the particle particle channels, this last integral is of order $w^2$ near the fixed points. This means that the polynomial \eqref{eq:betatpolynomial} will have a cubic term $t(\ell)^3$ with coefficient of order $w^2$. In the small $v$ limit, this term is negligible as will produce contributions of order $w$, $w^{3/2}$ and $w^{2}$ in the zeroes $t^*(\ell)$ of Eq. \eqref{eq:betatpolynomial}. By looking Eqs. \eqref{eq:etaevf}, \eqref{eq:Revf} and \eqref{eq:zedfeq}, we can clearly see that $t^*(\ell)$ has a leading order of $w^{1/2}$. Therefore, we can discard the $\left\langle f | \hat{\eta}^{(2)} | f \right\rangle$ term in Eq. \eqref{eq:etaevf}.

The zeroes of the polynomial in Eq. \eqref{eq:betatpolynomial} are
\begin{equation}
%\begin{aligned}
%&
t^*(\ell) = -\frac{4\pi\langle f | \eta | f \rangle}{\langle f | f \rangle} \pm \frac{2\pi}{\langle f | f \rangle}\sqrt{4\langle f | \eta | f \rangle^2 - \frac{2 Y^{(\pm)}_{PP}1^{\spmqty{s \\ d}}}{\pi N_f}\langle f | f \rangle\langle f |R| f \rangle}
%\\ & = -\frac{(N_c^2-1)}{N_c N_f}\left[\frac{\log\left(\frac{\Lambda}{2vc\varepsilon}\right)}{\log\left(\frac{\Delta}{\varepsilon}\right)}+ \frac{4}{\pi}\log\left(\frac{1}{c}\right) - 2\right]\frac{v}{c}
%\\ & \pm \frac{4\pi^2}{\log\left(\frac{\Delta}{\varepsilon}\right)}\sqrt{\frac{(N_c^2-1)^2}{\pi^2 N_c^2 N_f^2}\left[\frac{\log\left(\frac{\Lambda}{2 v c \varepsilon}\right)}{4\pi} + \left(\frac{2}{\pi}\log\left(\frac{1}{c}\right) -1 \right)\frac{1}{2\pi}\log\left(\frac{\Delta}{\varepsilon}\right) \right]^2 \frac{v^2}{c^2} - \frac{Y^{(\pm)}_{PP}1^{\spmqty{s \\ d}}}{8 \pi^2 N_f}\log\left(\frac{\Delta}{\varepsilon}\right)\frac{v}{c}\log\left(\frac{2}{v}\right)},
%\end{aligned}
\label{eq:quasifixedpoints}
\end{equation}
where the explicit expressions for the three different terms are given by Eqs. \eqref{eq:braketnotation}, \eqref{eq:Revf} and \eqref{eq:etaevfexplicit}. The reader should also recall the definitions of $1^{\spmqty{s \\ d}}$ and $Y_{PP}^{(\pm)}$, given in Eqs. \eqref{eq:1sd} and \eqref{eq:Ypm}, respectively.

\begin{figure}[t]
\centering
\includegraphics[width=0.4\linewidth]{./Figures/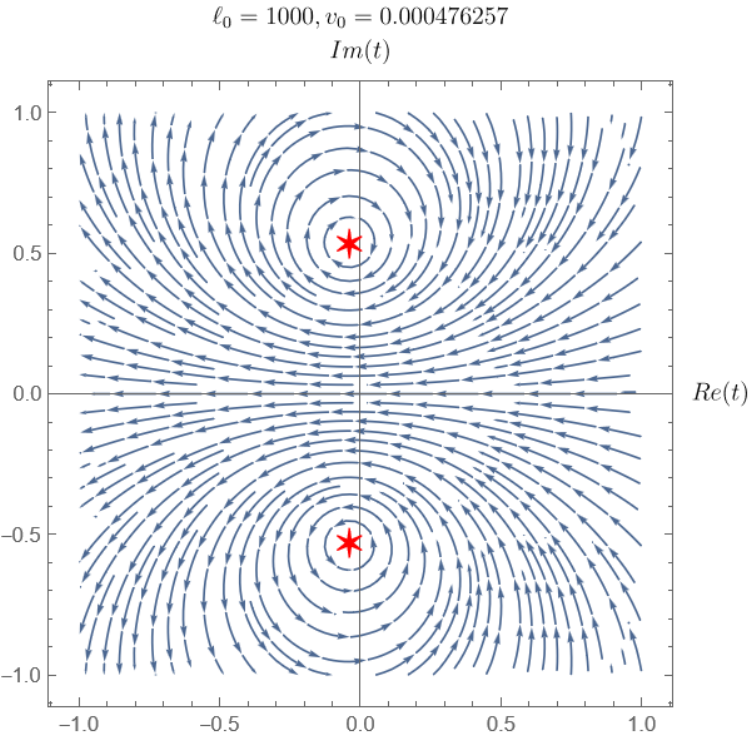}
\includegraphics[width=0.4\linewidth]{./Figures/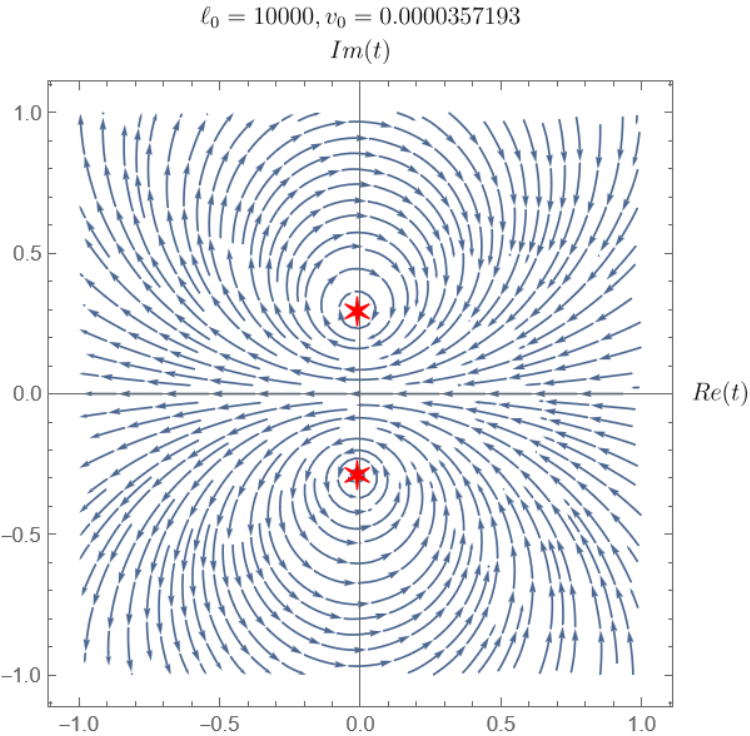}\\
\includegraphics[width=0.4\linewidth]{./Figures/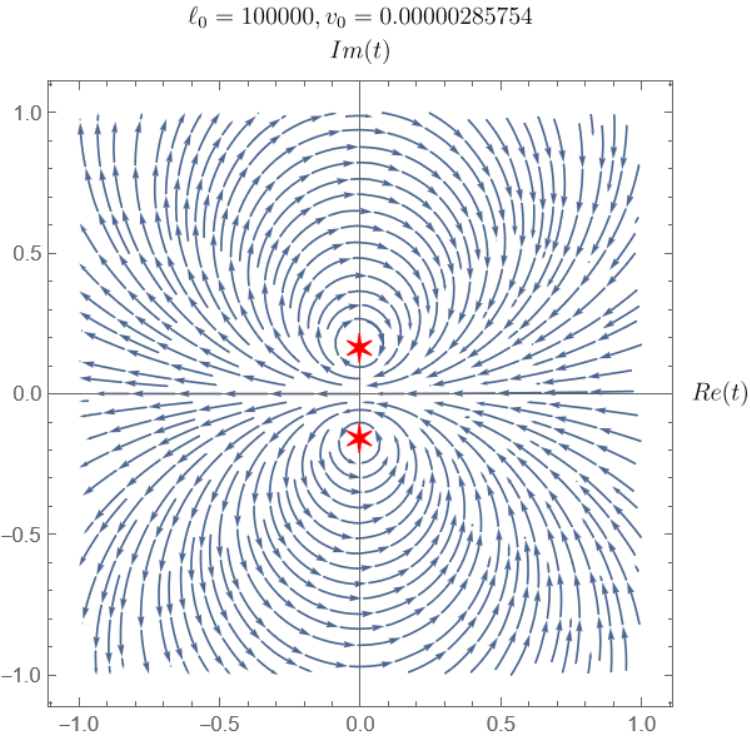}
\includegraphics[width=0.4\linewidth]{./Figures/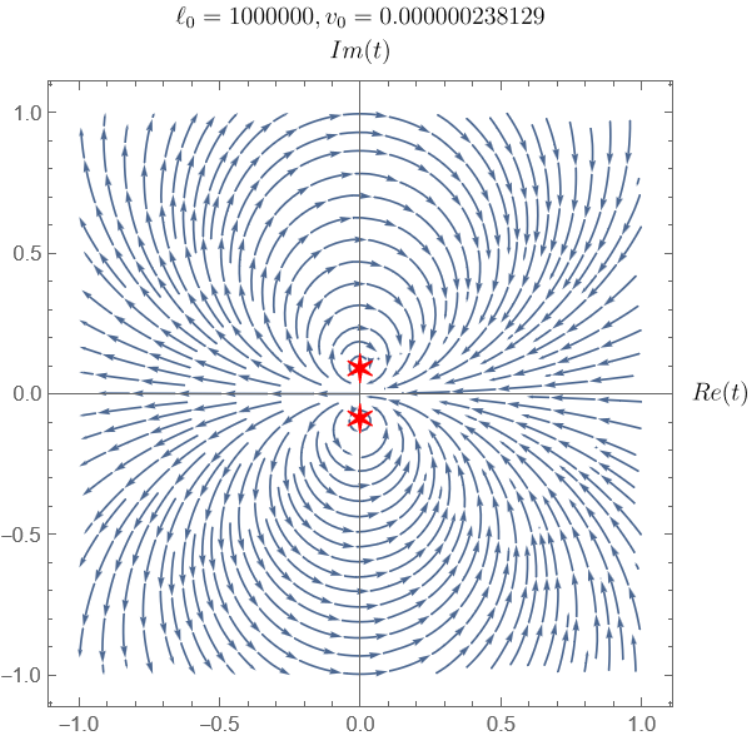}
\caption{Quasi-fixed point of Eq. \eqref{eq:betatpolynomial}, for increasing values of $\ell_0$ in the $(-,d)$ channel with $N_c = 2, N_f = 1$. The quasi-fixed points themselves are marked as red six pointed stars. Here we have chosen $\Delta = \Lambda, \varepsilon = 10^{-100} \Delta$ ($\Lambda$ is ormalized to 1). The top two figures show the vector flow for $\ell_0 = 1000, 10000$, from left to right. The bottom two plots correspond to $\ell_0 = 100000, 1000000$.}
\label{fig:streamflow}
\end{figure}
Consider the case of $n = (-,d)$, i.e. $Y_{PP}^{(-)} = -2\left(\frac{1}{N_c}+1 \right)$ and $1^{\spmqty{s \\ d}} = -1$ . The flow of Eq. \eqref{eq:betatpolynomial} is depicted in Fig. \ref{fig:streamflow} for increasing values of $\ell_0$ with $\ell = 0$. In the last equation, the quasi-fixed points are achieved because the discriminant in the square root is negative for $0 < \varepsilon \ll \Delta$, making the second term of the equation imaginary. The flow of this ``beta'' function (projection) is formed by closed orbit. If we perturb around the fixed points as
\begin{equation}
t(\ell) = t^*(\ell) + \delta t(\ell),
\label{eq:tperturbation}
\end{equation}
we obtain an imaginary $t$-independent value for each point:
\begin{equation}
%\begin{aligned}
%& 
\frac{\partial\delta t(\ell)}{\partial\ell} =  -\left.\frac{\partial\beta^{(t)}}{\partial z}\right\rvert_{t^*}\delta t(\ell) = \pm \frac{2\pi}{\langle f | f \rangle}\sqrt{4\langle f | \eta | f \rangle^2 - \frac{4}{\pi N_f}\left(\frac{1}{N_c}+1 \right)\langle f | f \rangle\langle f |R| f \rangle}\delta t(\ell).
%\end{aligned}
\end{equation}
We can see the orbits in Fig. \ref{fig:streamflow}. As the last equation suggests, these are closed orbits to fisrt order, as the rate of change of the beta function with respect to the ``coupling'' $t$, is purely imaginary near the fixed points, i.e.
\begin{equation}
\delta t(\ell) = \delta t(0) \exp\left\lbrace\pm i \frac{2\pi}{\langle f | f \rangle}\sqrt{\abs{4\langle f | \eta | f \rangle^2 - \frac{4}{\pi N_f}\left(\frac{1}{N_c}+1 \right)\langle f | f \rangle\langle f |R| f \rangle }}\right\rbrace,
\end{equation}
which is a circular orbit around the fixed point (labeled by $\pm$.)

In Fig. \ref{fig:streamflow} the function in which the quasi-fixed points approach the axis of real theories as a function of $v_0$ is determined by Eq. \eqref{eq:quasifixedpoints}. This equation gives a real value of $t^*$ asymptotically in the limit $v_0 \xrightarrow[\ell_0 \to \infty]{} 0$, as expected, but for finite values of $v_0$ the fixed points flow to the real axis increasingly slowly, never reaching the space of Hermitian theories.
